# Supplementary material for: Exploring the Impact of Imaging Cadence on Inferring CME Kinematics
Source: arXiv:2308.11944 source file (2023-08-23)
Supplement: Supplementary file 1 [file supplementary_material.pdf]

# Supplementary Material

## 1 DISTRIBUTION OF VELOCITY AND ACCELERATION

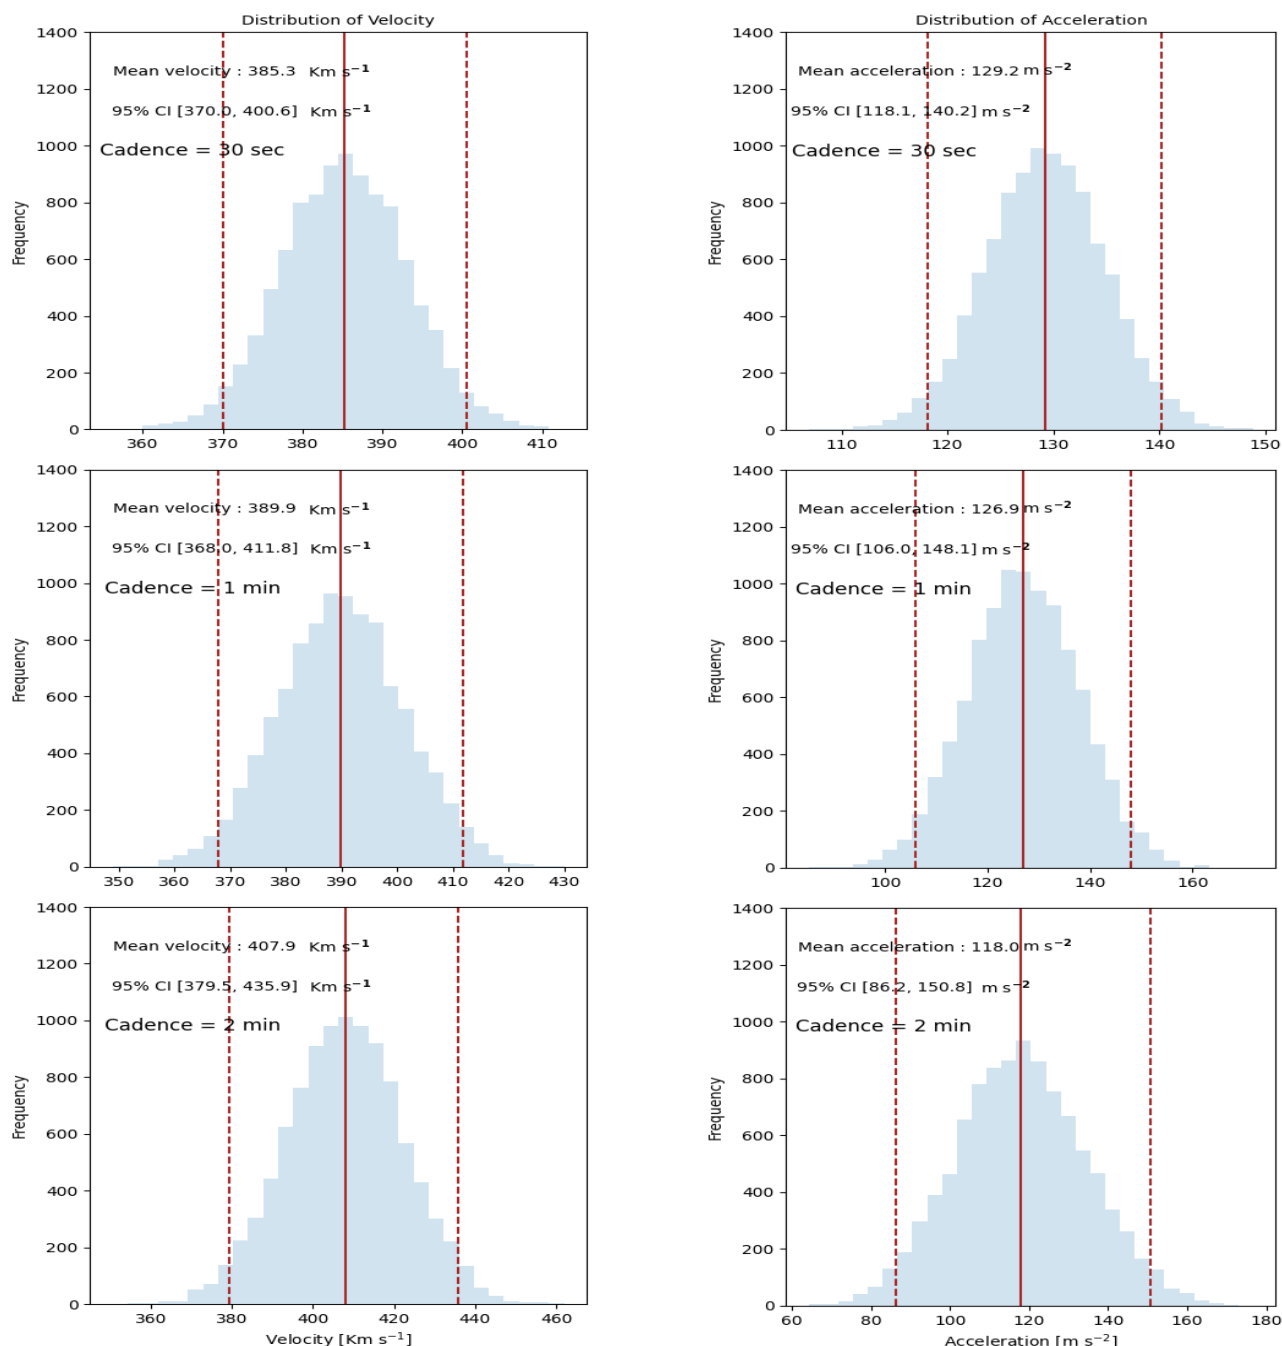

**Figure S1.** Histograms depicting the distribution of velocity (left column) and acceleration (right column) values obtained using the linear fit and quadratic fit method, respectively, with the application of the bootstrapping technique for the CME occurred on November 05, 2014. The dashed and solid line represents the 95% confidence interval and mean of the distribution, respectively.

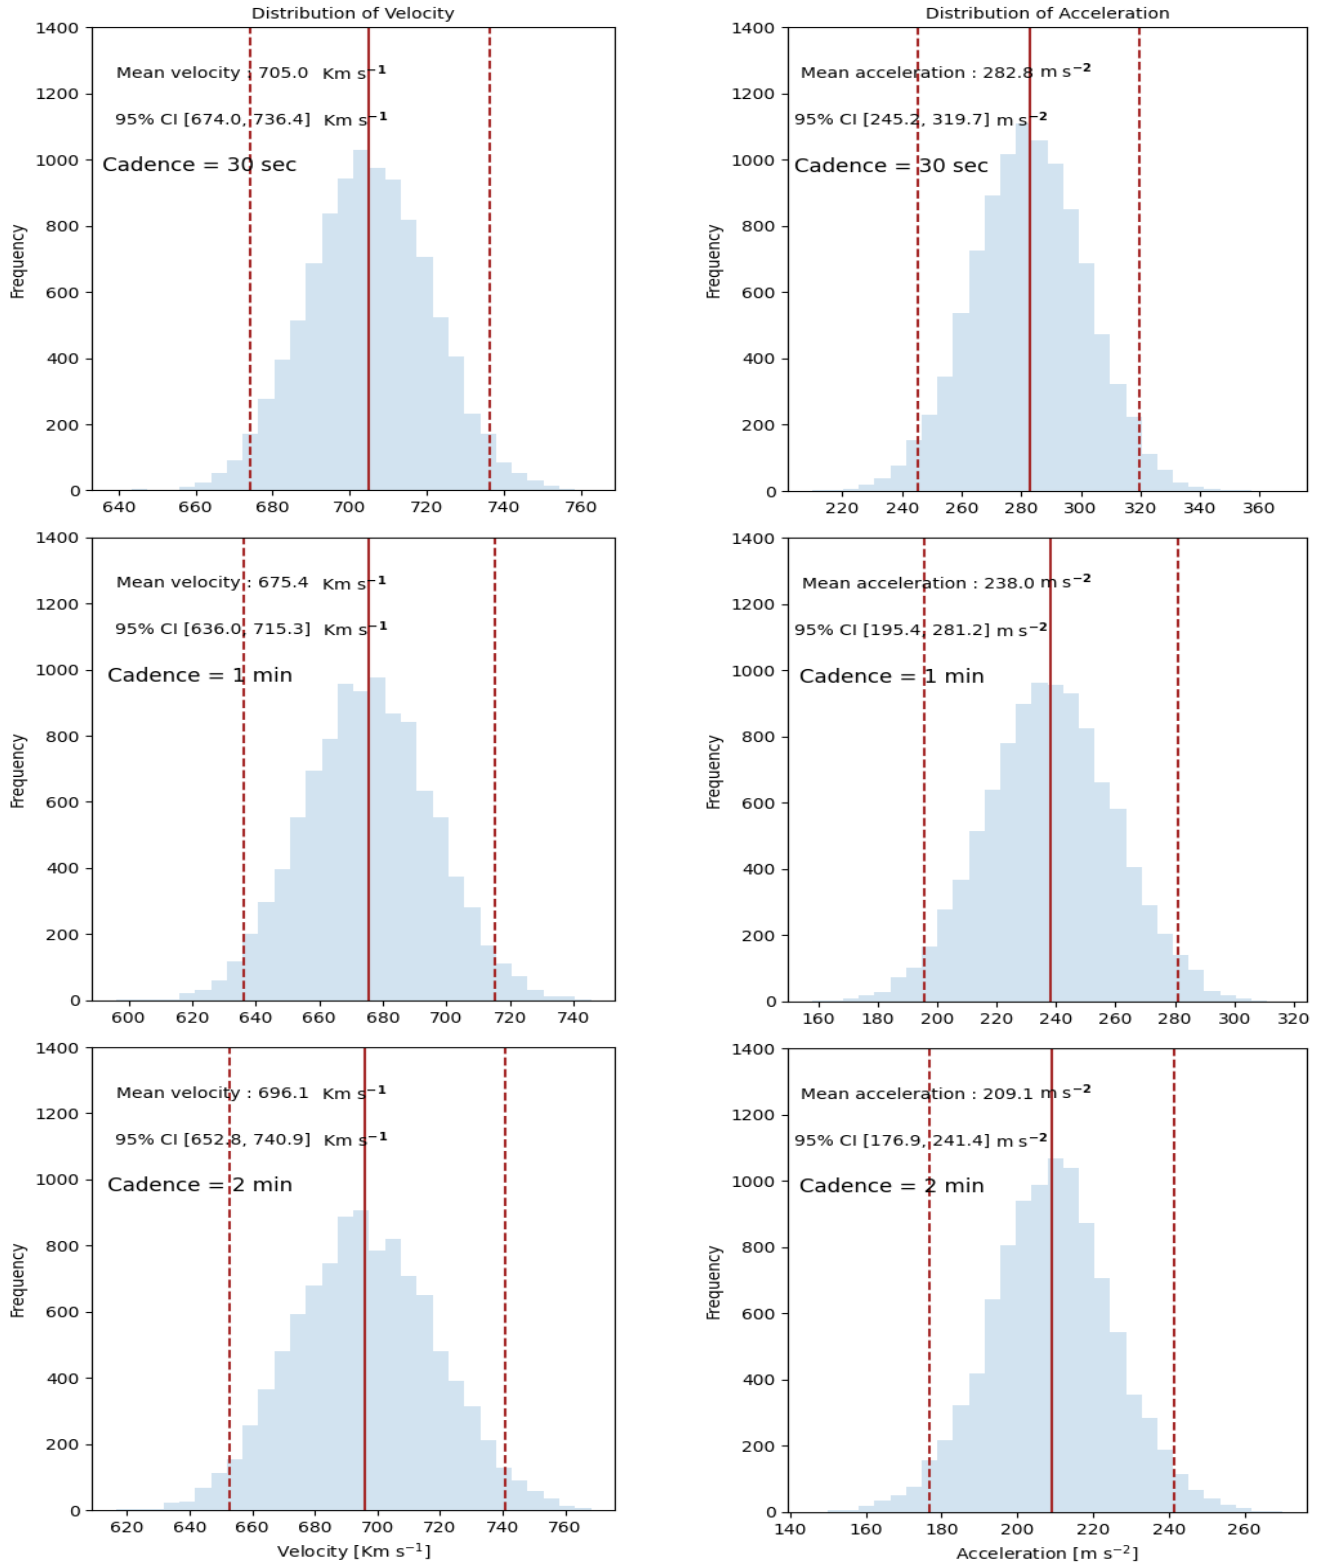

**Figure S2.** Histograms depicting the distribution of velocity (left column) and acceleration (right column) values obtained using the linear fit and quadratic fit method, respectively, with the application of the bootstrapping technique for the CME occurred on May 07, 2021. The dashed and solid line represents the 95% confidence interval and mean of the distribution, respectively.

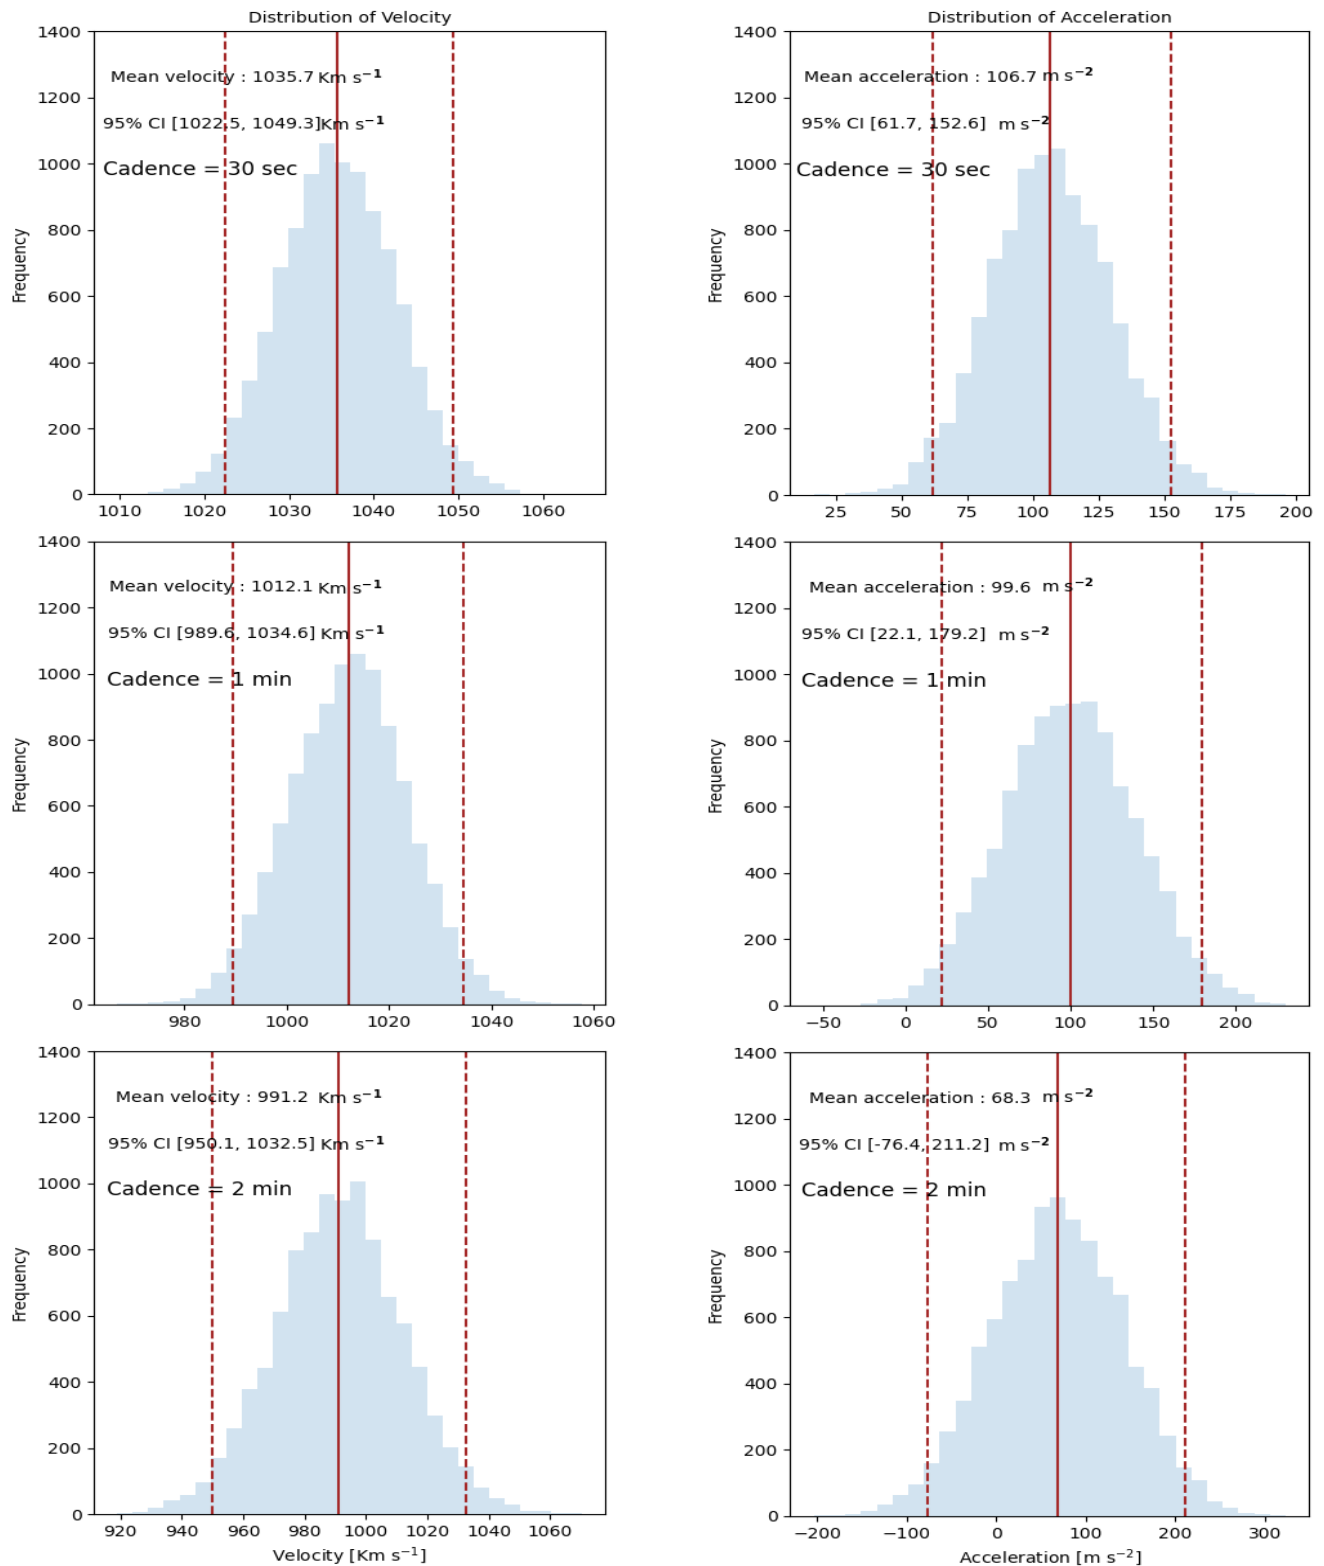

**Figure S3.** Histograms depicting the distribution of velocity (left column) and acceleration (right column) values obtained using the linear fit and quadratic fit method, respectively, with the application of the bootstrapping technique for the CME occurred on July 15, 2021. The dashed and solid line represents the 95% confidence interval and mean of the distribution, respectively.

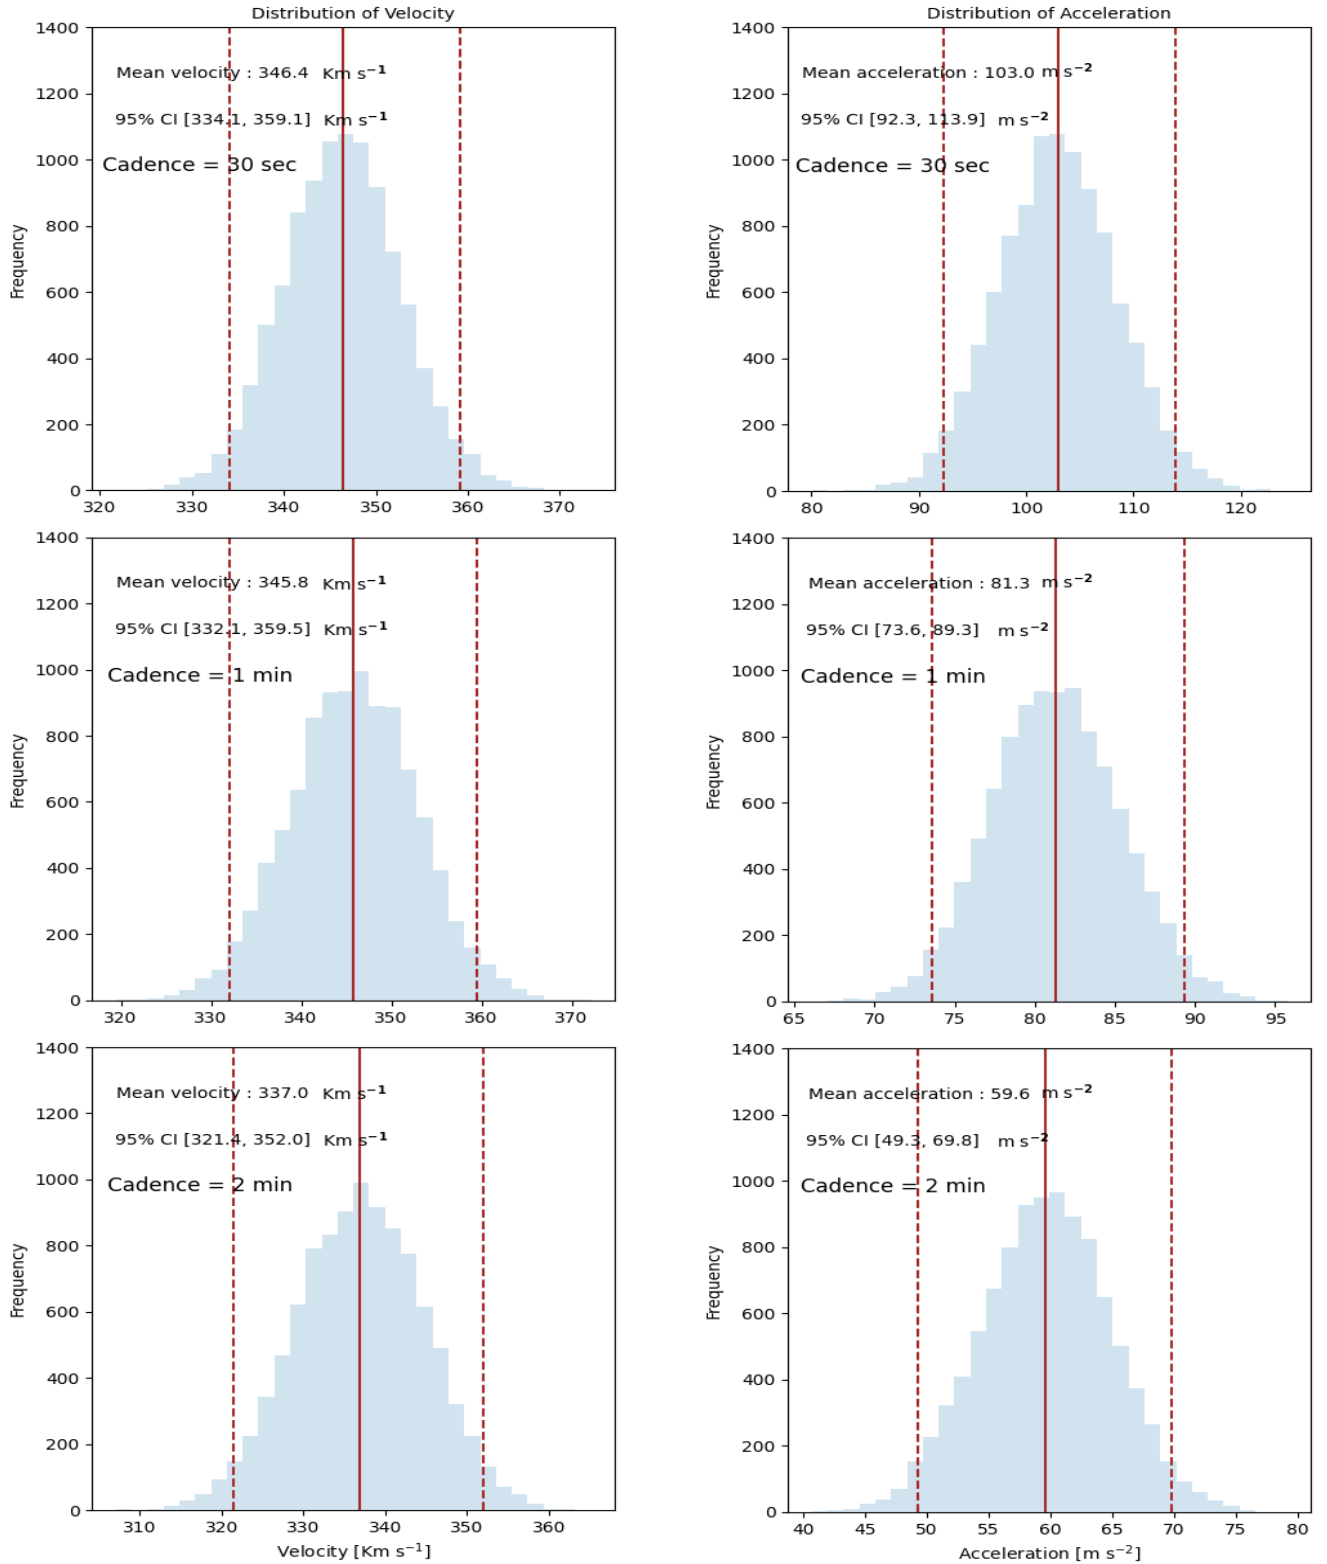

**Figure S4.** Histograms depicting the distribution of velocity (left column) and acceleration (right column) values obtained using the linear fit and quadratic fit method, respectively, with the application of the bootstrapping technique for the CME occurred on October 10, 2021. The dashed and solid line represents the 95% confidence interval and mean of the distribution, respectively.

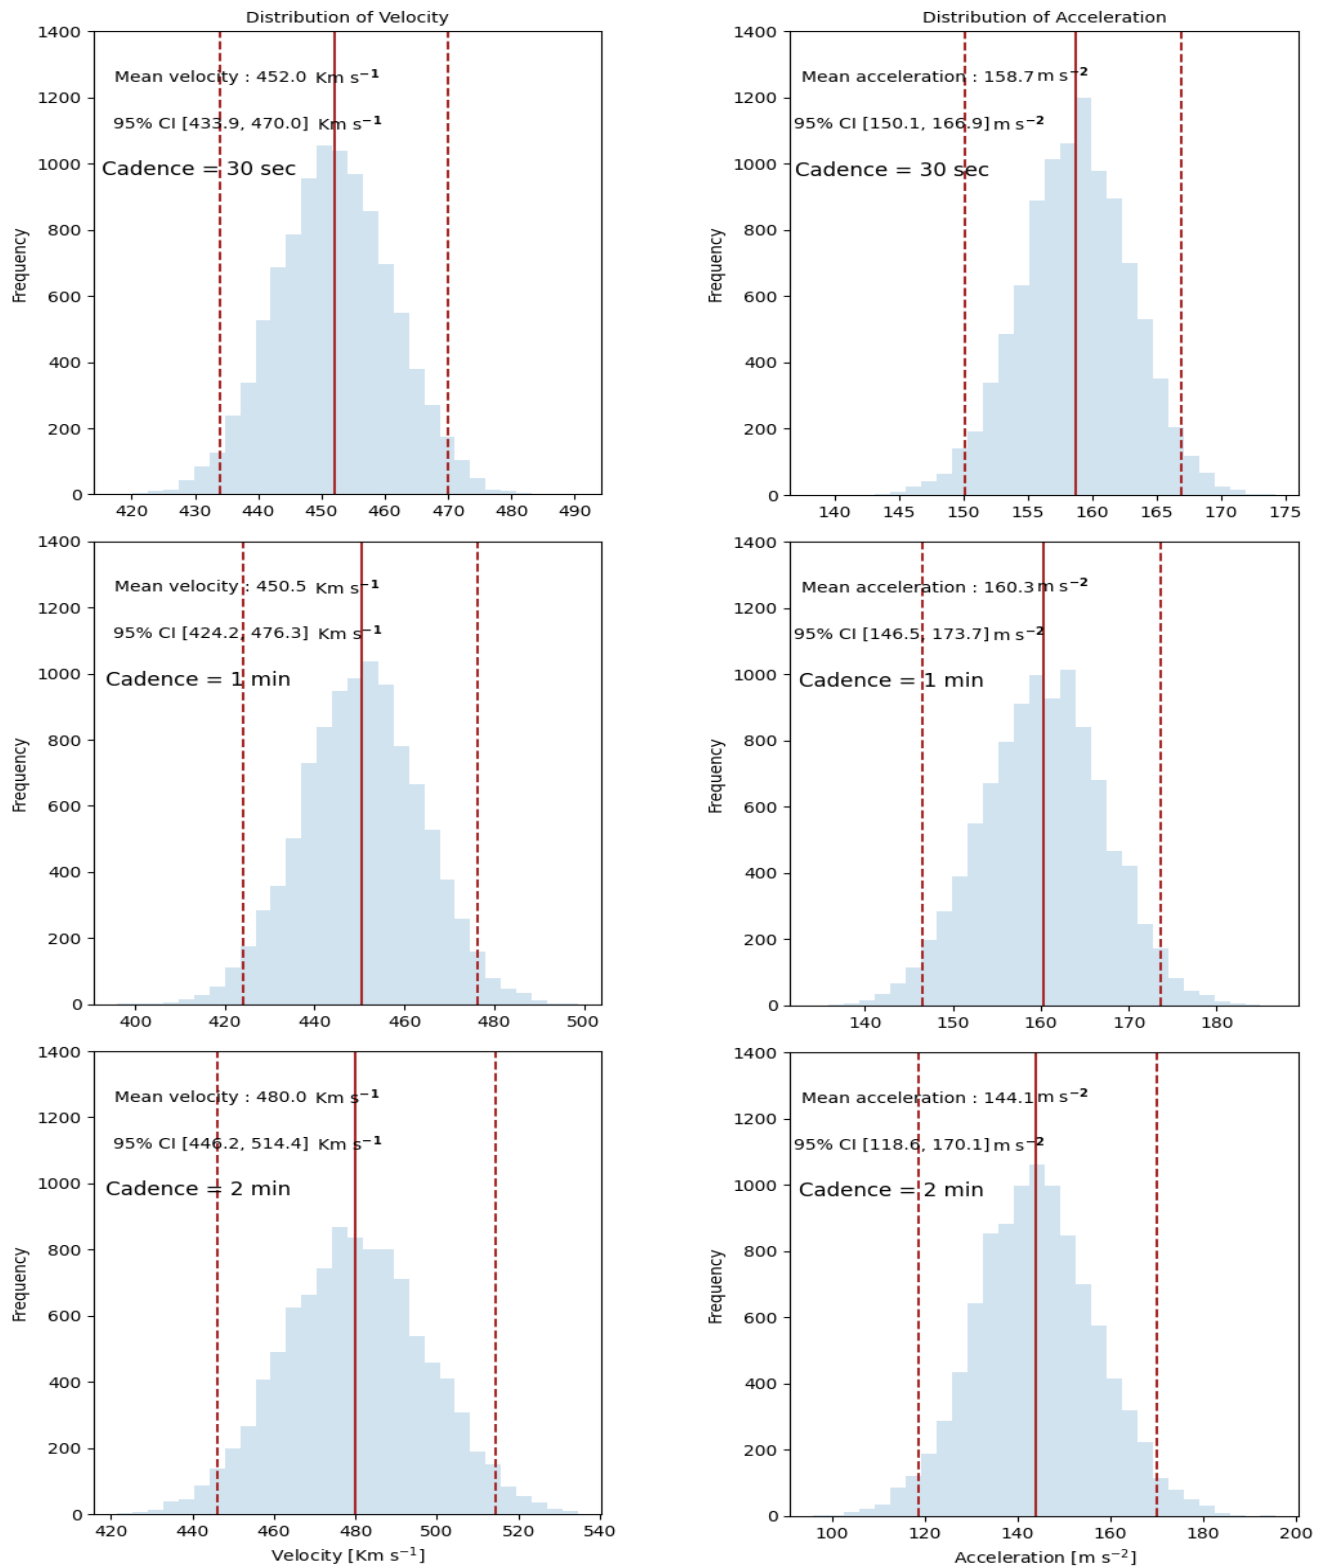

**Figure S5.** Histograms depicting the distribution of velocity (left column) and acceleration (right column) values obtained using the linear fit and quadratic fit method, respectively, with the application of the bootstrapping technique for the CME occurred on January 10, 2022. The dashed and solid line represents the 95% confidence interval and mean of the distribution, respectively.

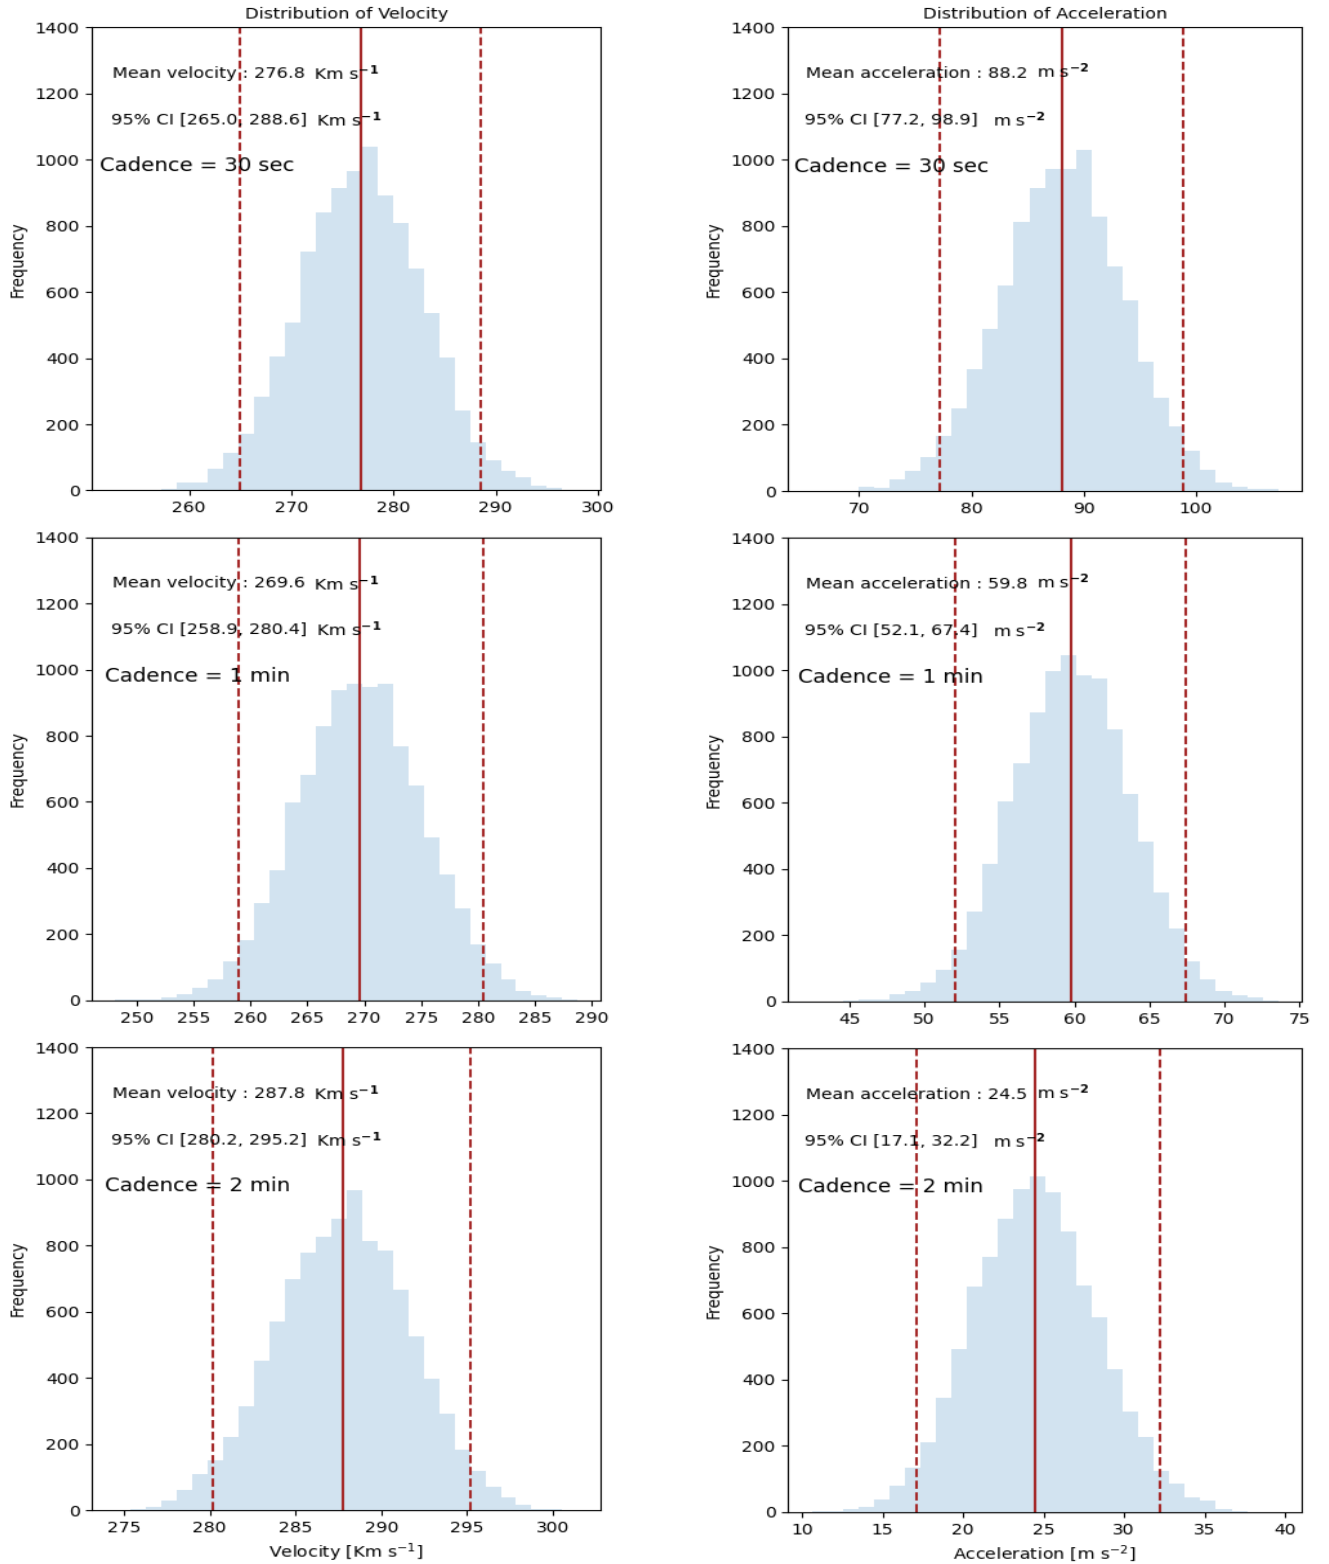

**Figure S6.** Histograms depicting the distribution of velocity (left column) and acceleration (right column) values obtained using the linear fit and quadratic fit method, respectively, with the application of the bootstrapping technique for the CME occurred on May 08, 2022. The dashed and solid line represents the 95% confidence interval and mean of the distribution, respectively.

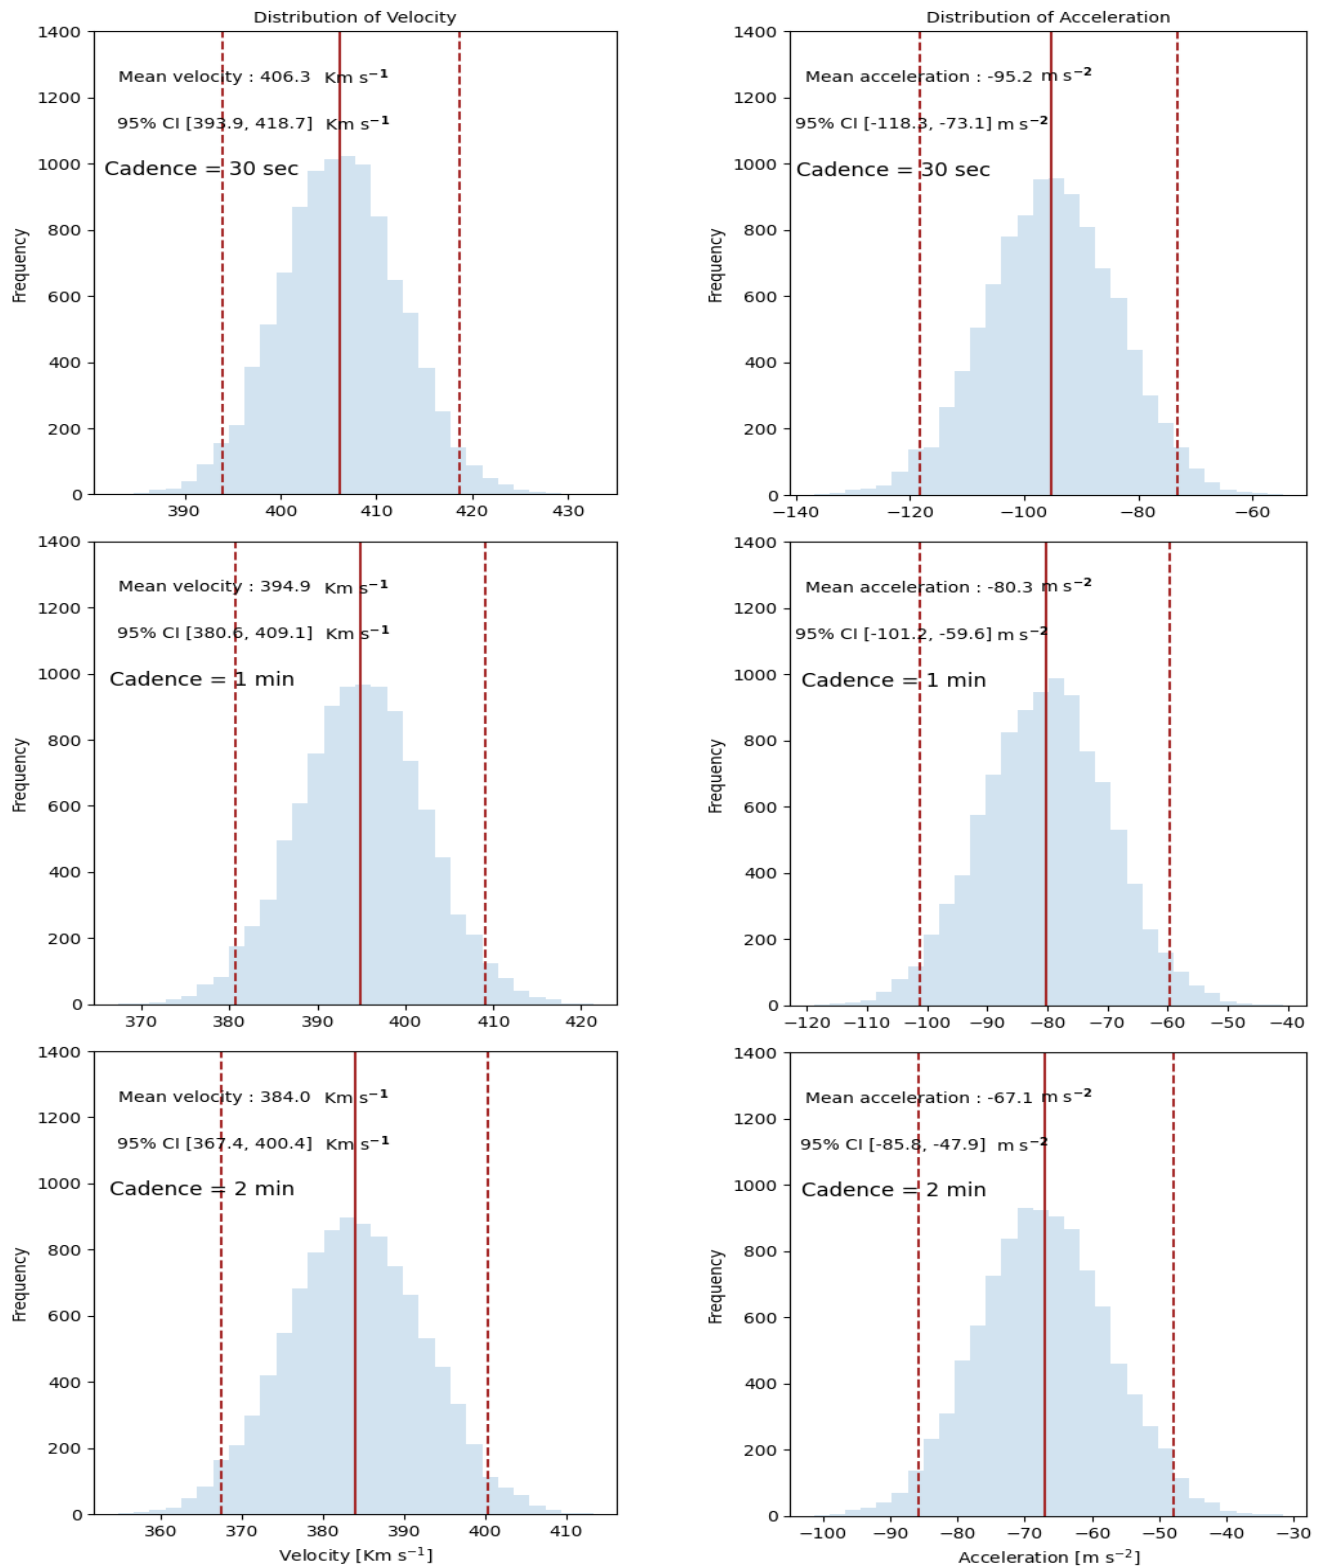

**Figure S7.** Histograms depicting the distribution of velocity (left column) and acceleration (right column) values obtained using the linear fit and quadratic fit method, respectively, with the application of the bootstrapping technique for the CME occurred on May 24, 2022. The dashed and solid line represents the 95% confidence interval and mean of the distribution, respectively.

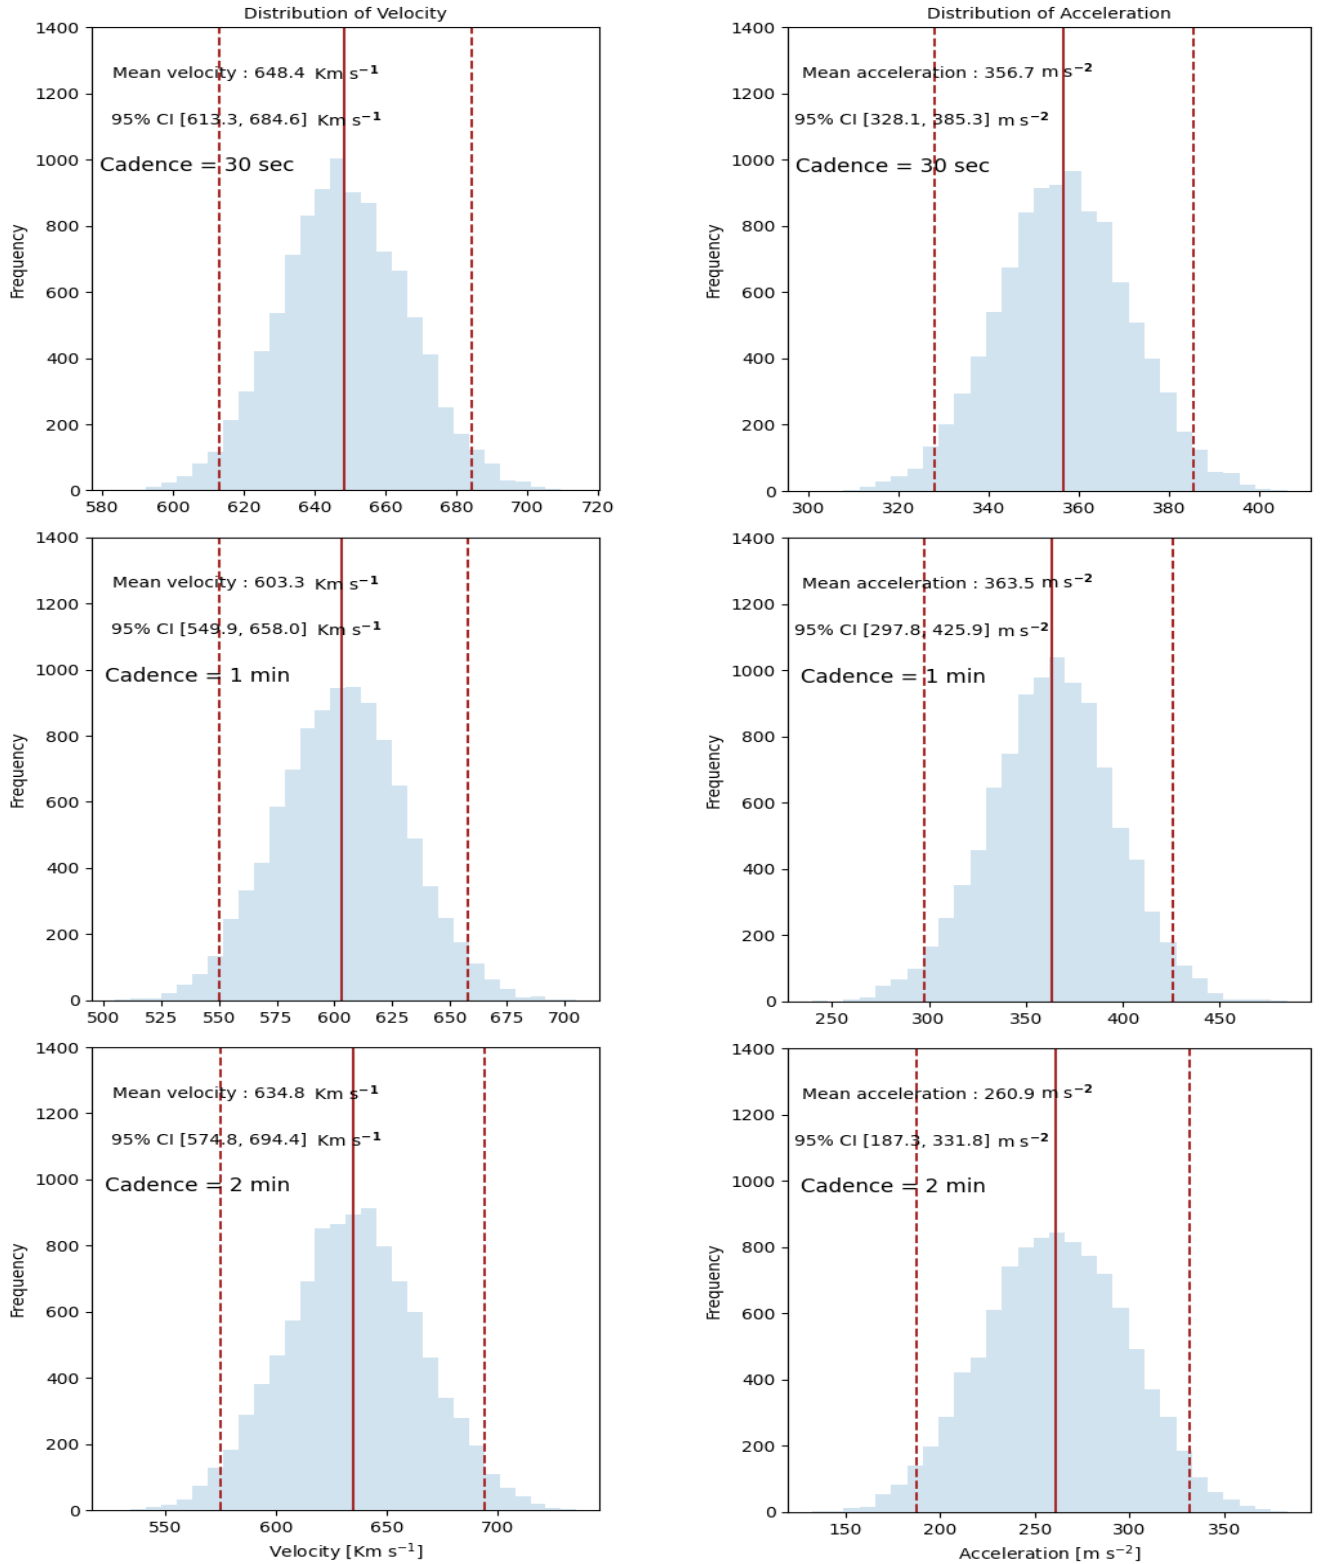

**Figure S8.** Histograms depicting the distribution of velocity (left column) and acceleration (right column) values obtained using the linear fit and quadratic fit method, respectively, with the application of the bootstrapping technique for the CME occurred on July 31, 2022. The dashed and solid line represents the 95% confidence interval and mean of the distribution, respectively.



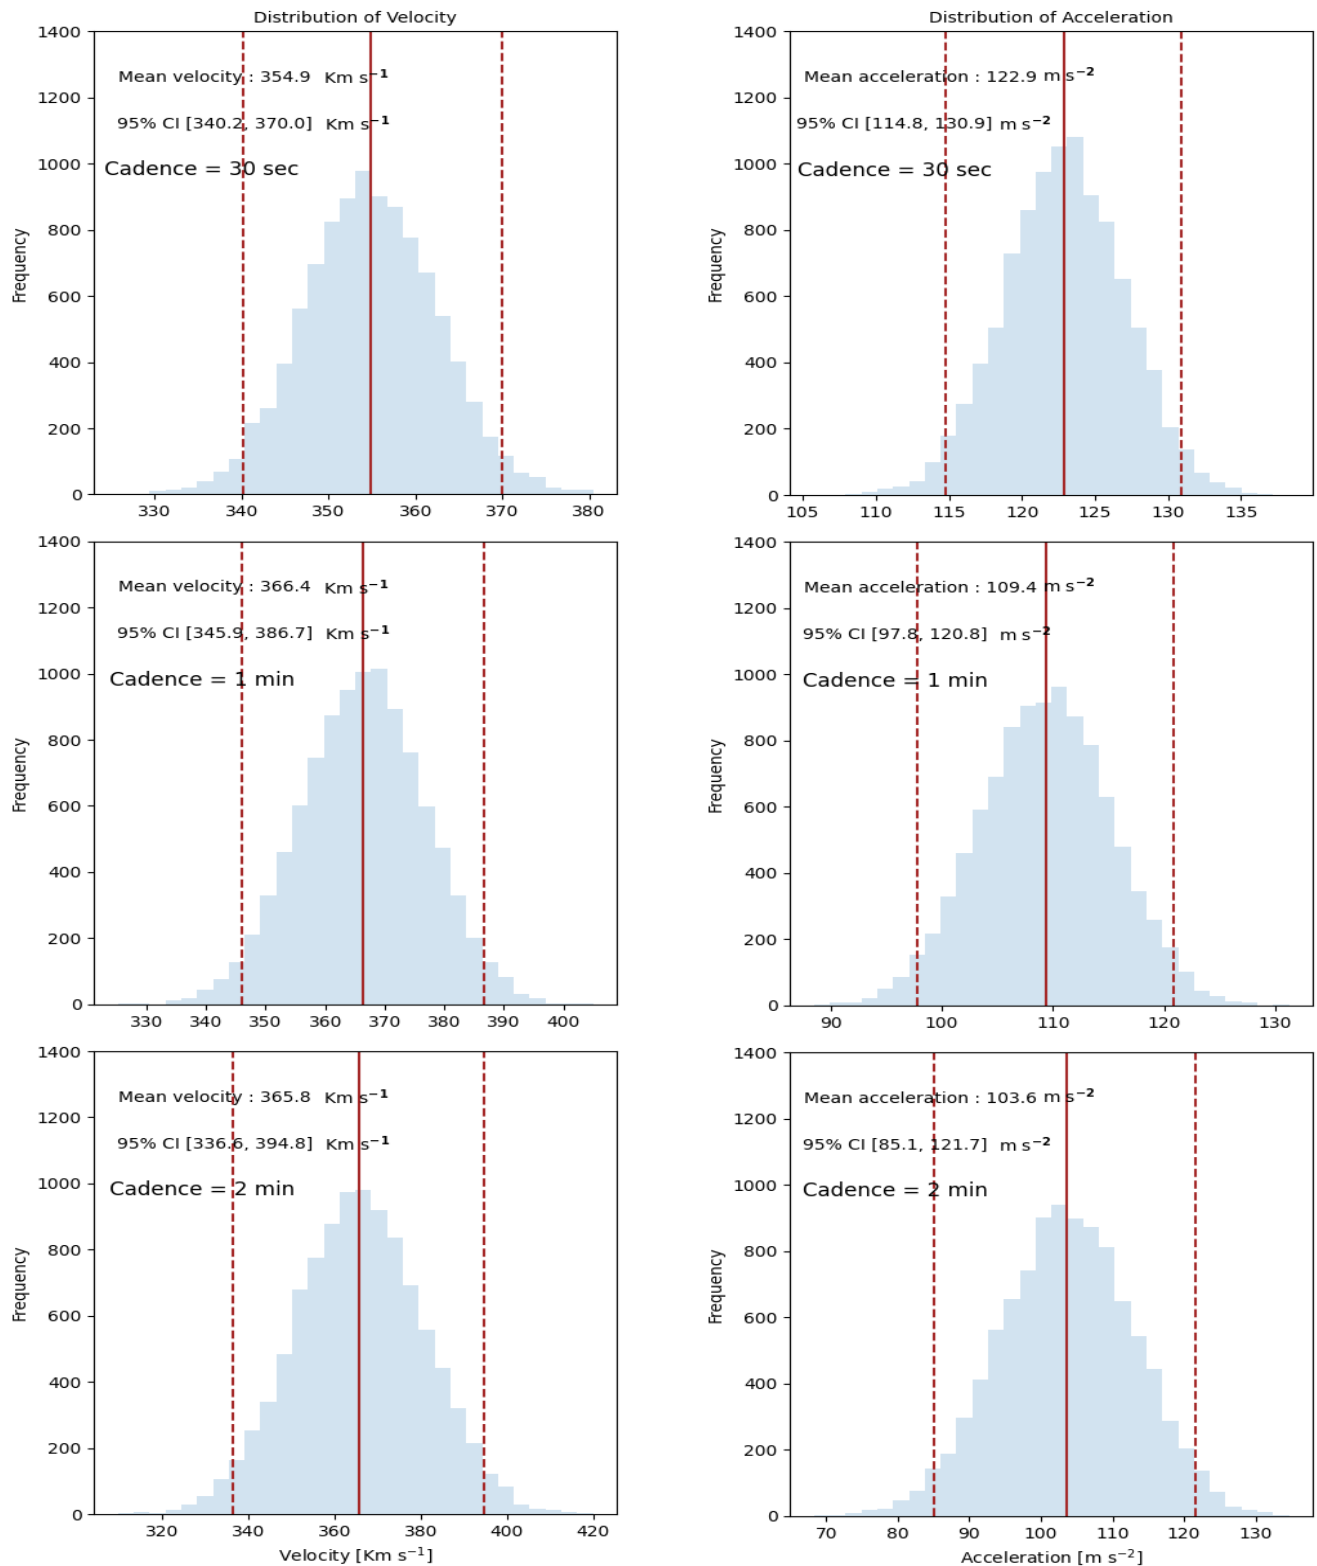

**Figure S9.** Histograms depicting the distribution of velocity (left column) and acceleration (right column) values obtained using the linear fit and quadratic fit method, respectively, with the application of the bootstrapping technique for the CME occurred on September 02, 2022. The dashed and solid line represents the 95% confidence interval and mean of the distribution, respectively.

## 2 HEIGHT-TIME PLOTS OF ALL THE CME EVENTS

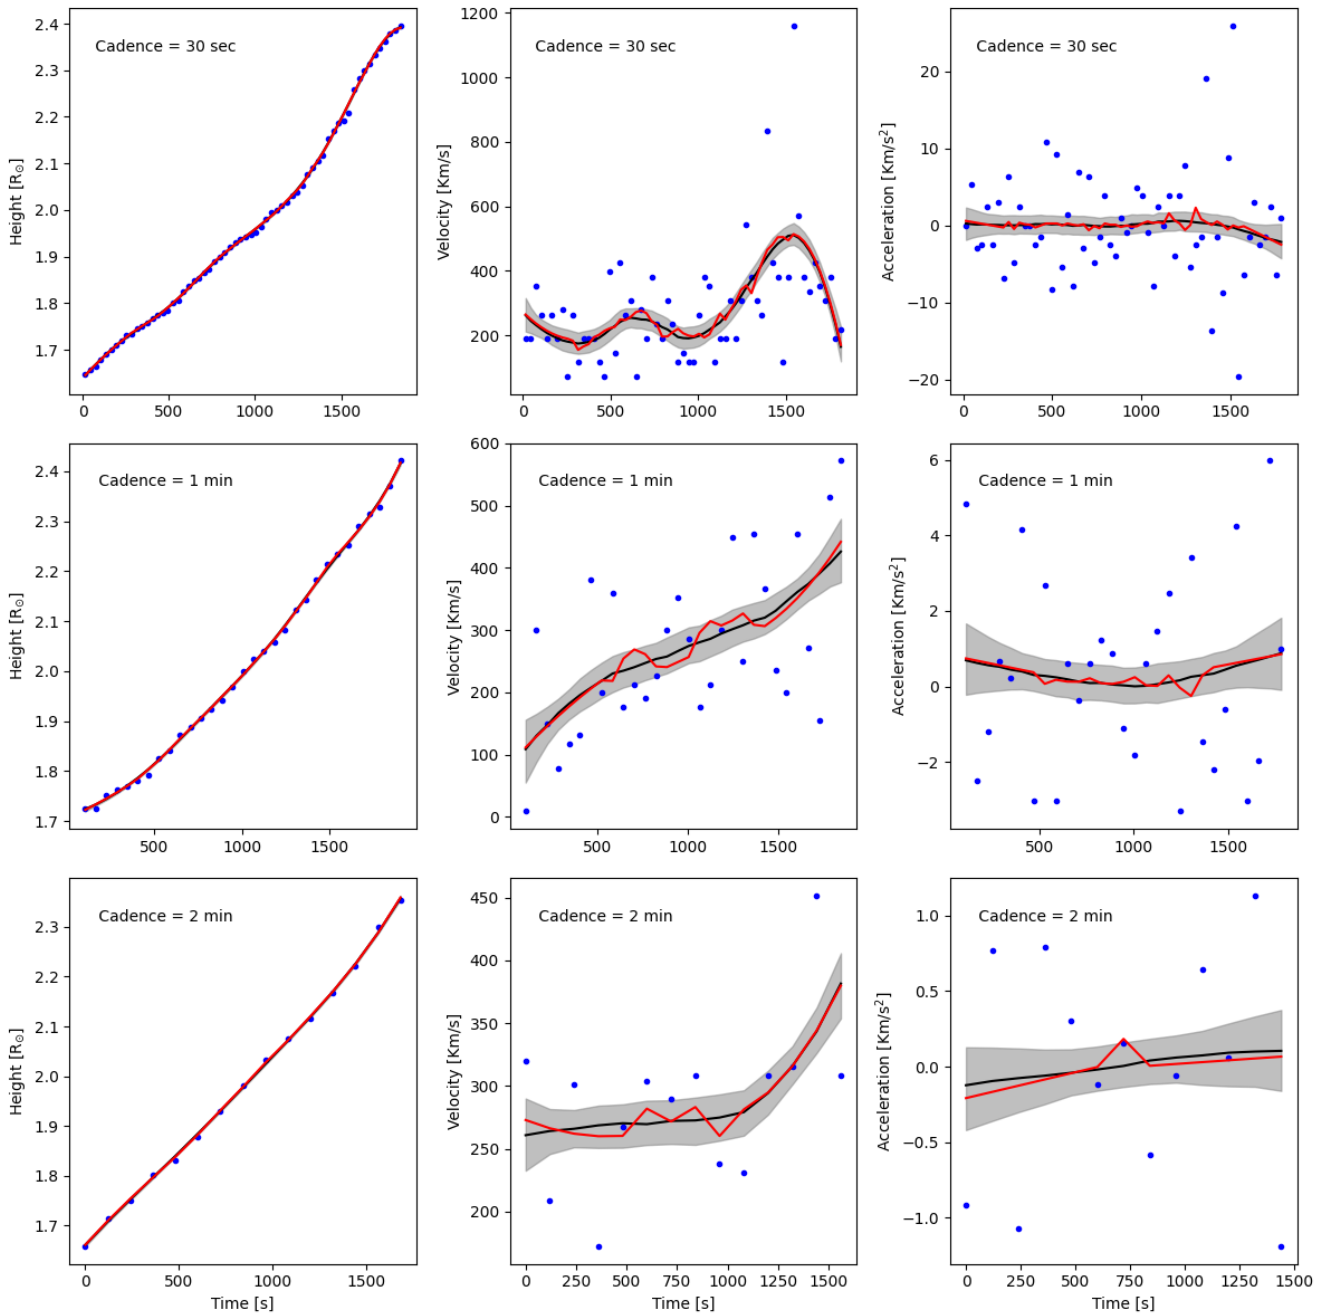

**Figure S10.** A complete kinematic profile of the CME observed on May 08, 2022. (a) represents the bootstrapped Savitzky-Golay filter applied height-time plot for each cadence (from top to bottom). (b) and (c) represents the corresponding velocity and acceleration plot, respectively. The blue dot represents (a) the height measurement taken using K-Cor coronagraph and (b) and (c) corresponding numerically derivative velocity and acceleration. The red line represents the fitted curve. The black line represents the median value, and the grey-shaded region depicts the interquartile range.

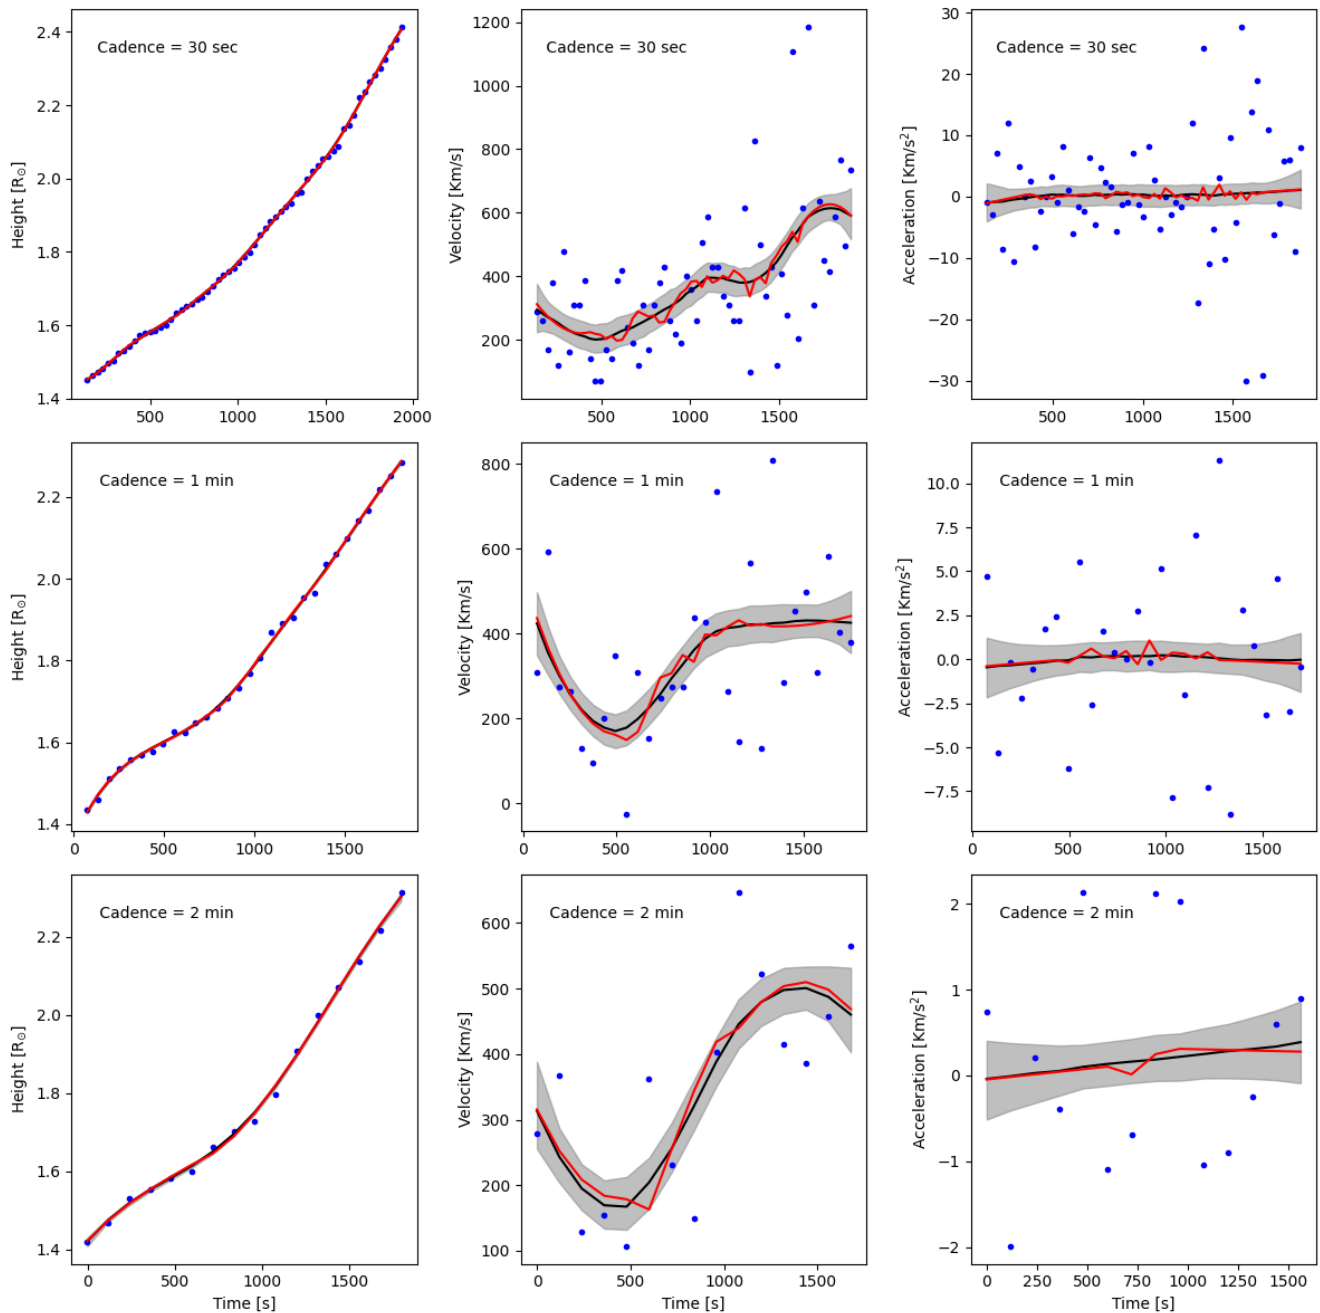

**Figure S11.** A complete kinematic profile of the CME observed on September 02, 2022. (a) represents the bootstrapped Savitzky-Golay filter applied height-time plot for each cadence (from top to bottom). (b) and (c) represents the corresponding velocity and acceleration plot, respectively. The blue dot represents (a) the height measurement taken using K-Cor coronagraph and (b) and (c) corresponding numerically derivative velocity and acceleration. The red line represents the fitted curve. The black line represents the median value, and the grey-shaded region depicts the interquartile range.

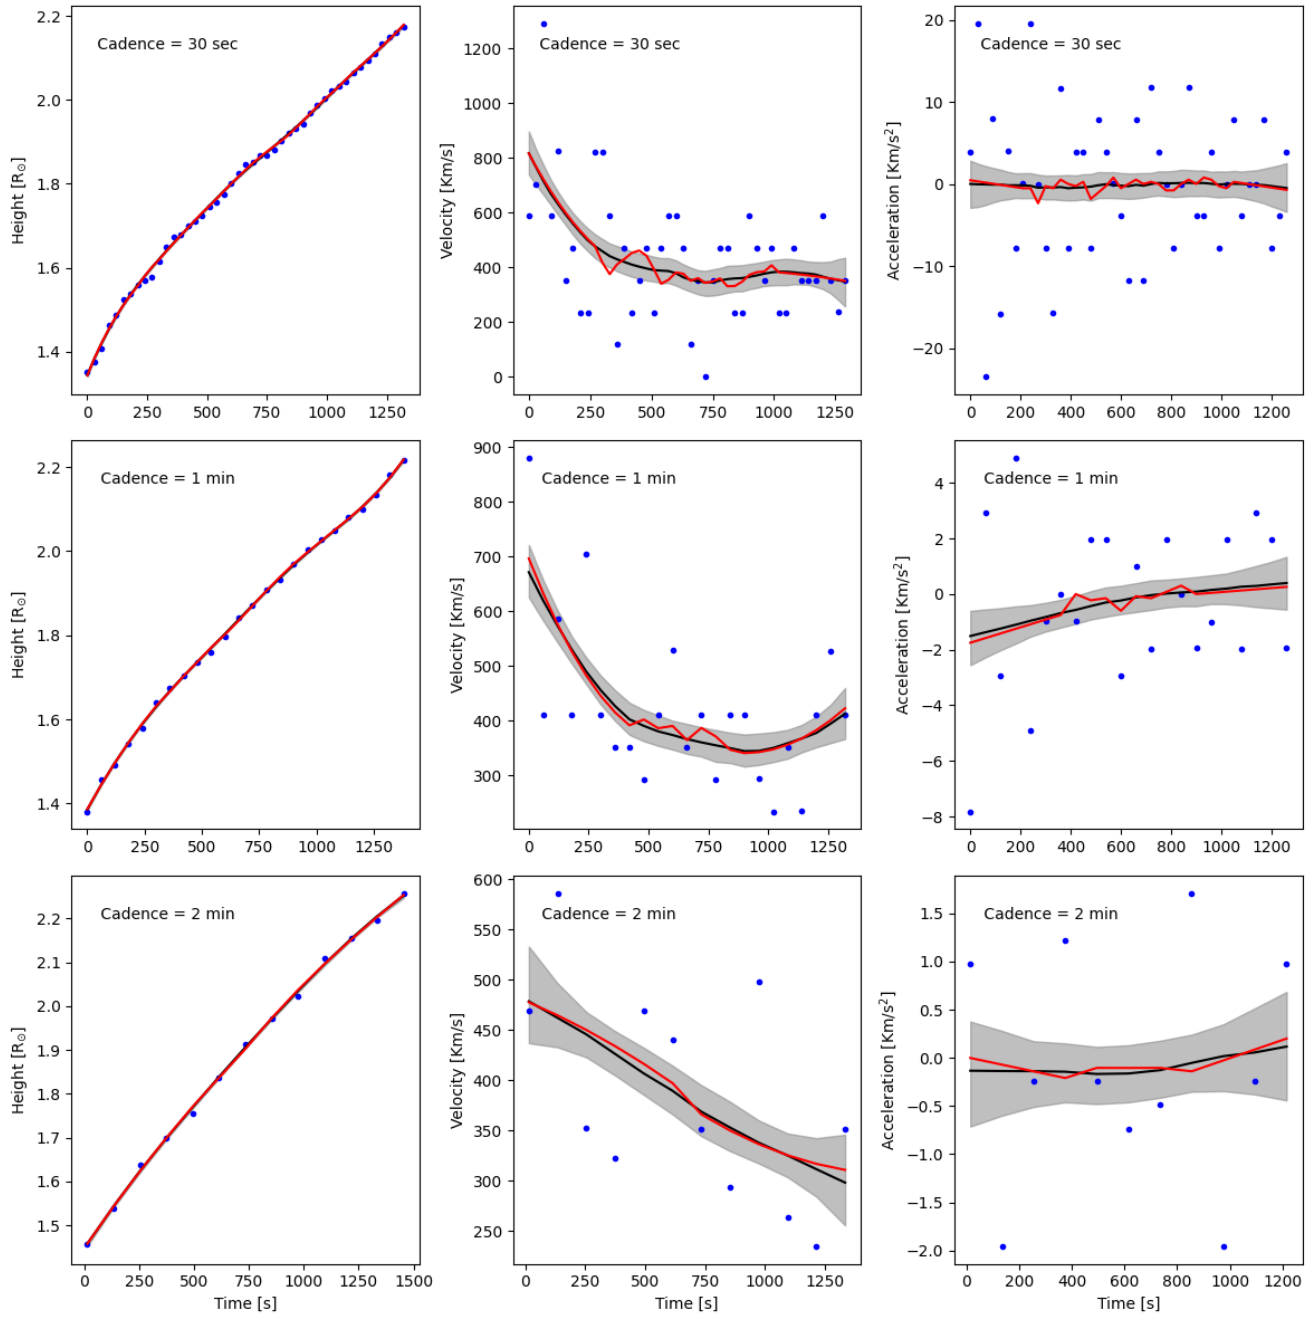

**Figure S12.** A complete kinematic profile of the CME observed on May 24, 2022. (a) represents the bootstrapped Savitzky-Golay filter applied height-time plot for each cadence (from top to bottom). (b) and (c) represents the corresponding velocity and acceleration plot, respectively. The blue dot represents (a) the height measurement taken using K-Cor coronagraph and (b) and (c) corresponding numerically derivative velocity and acceleration. The red line represents the fitted curve. The black line represents the median value, and the grey-shaded region depicts the interquartile range.

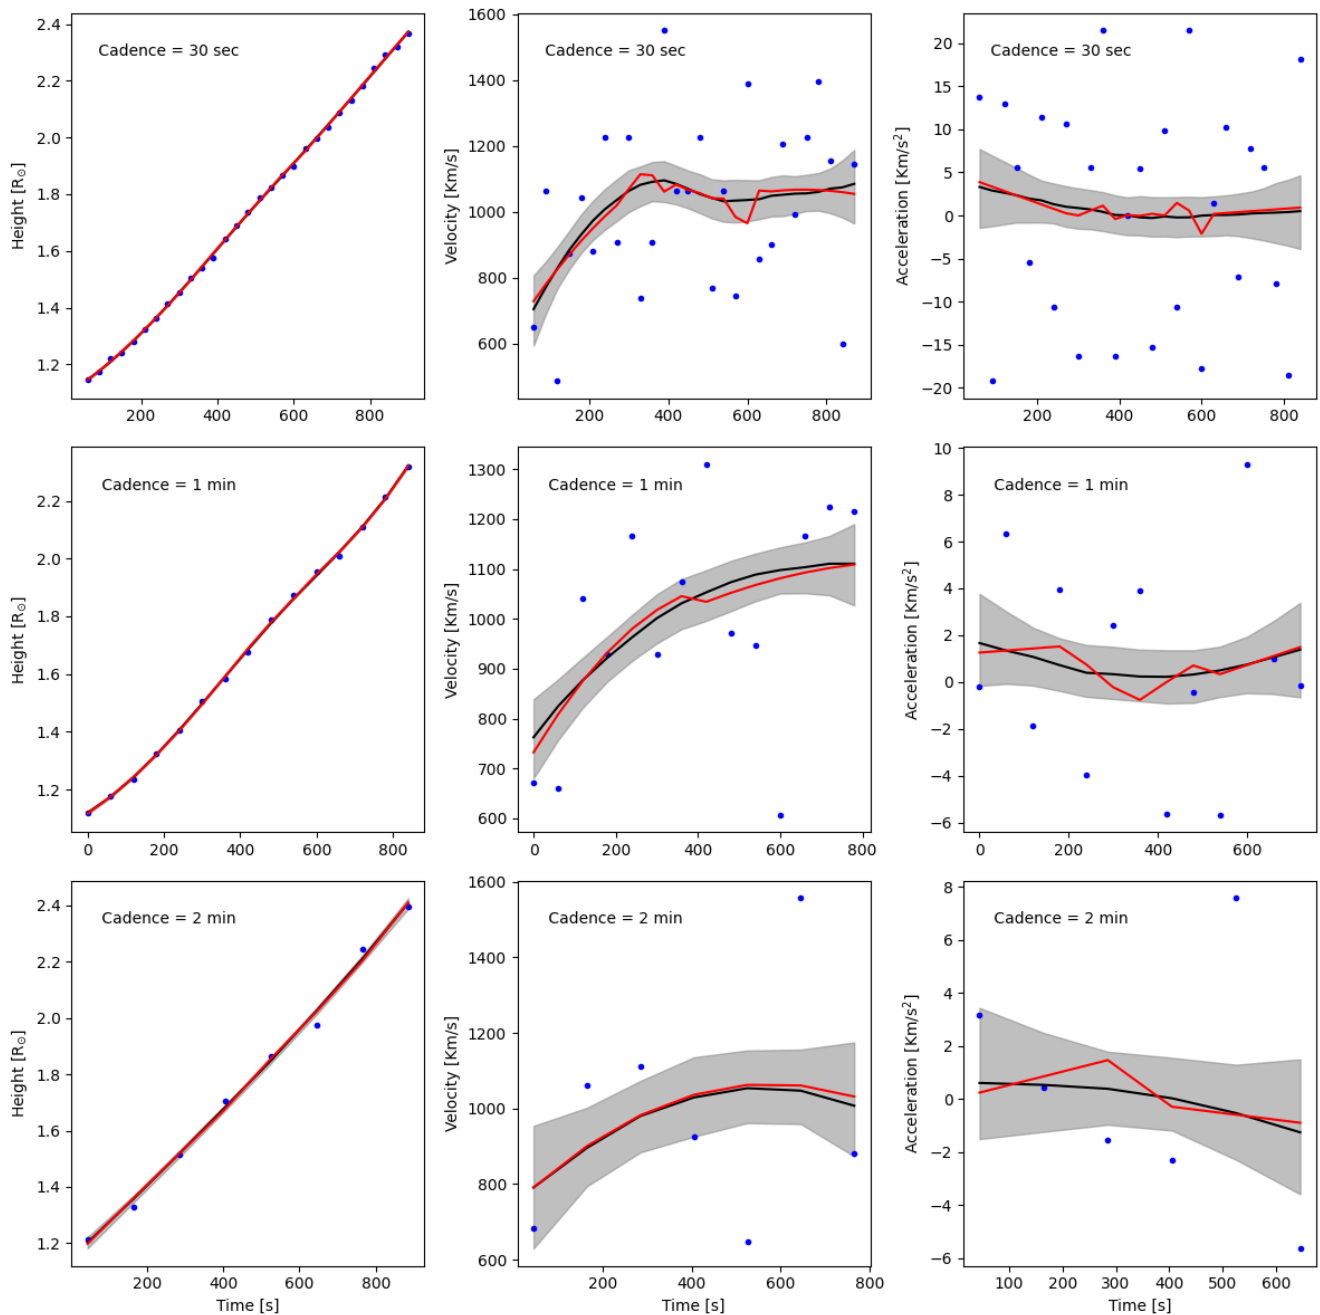

**Figure S13.** A complete kinematic profile of the CME observed on July 15, 2021. (a) represents the bootstrapped Savitzky-Golay filter applied height-time plot for each cadence (from top to bottom). (b) and (c) represents the corresponding velocity and acceleration plot, respectively. The blue dot represents (a) the height measurement taken using K-Cor coronagraph and (b) and (c) corresponding numerically derivative velocity and acceleration. The red line represents the fitted curve. The black line represents the median value, and the grey-shaded region depicts the interquartile range.

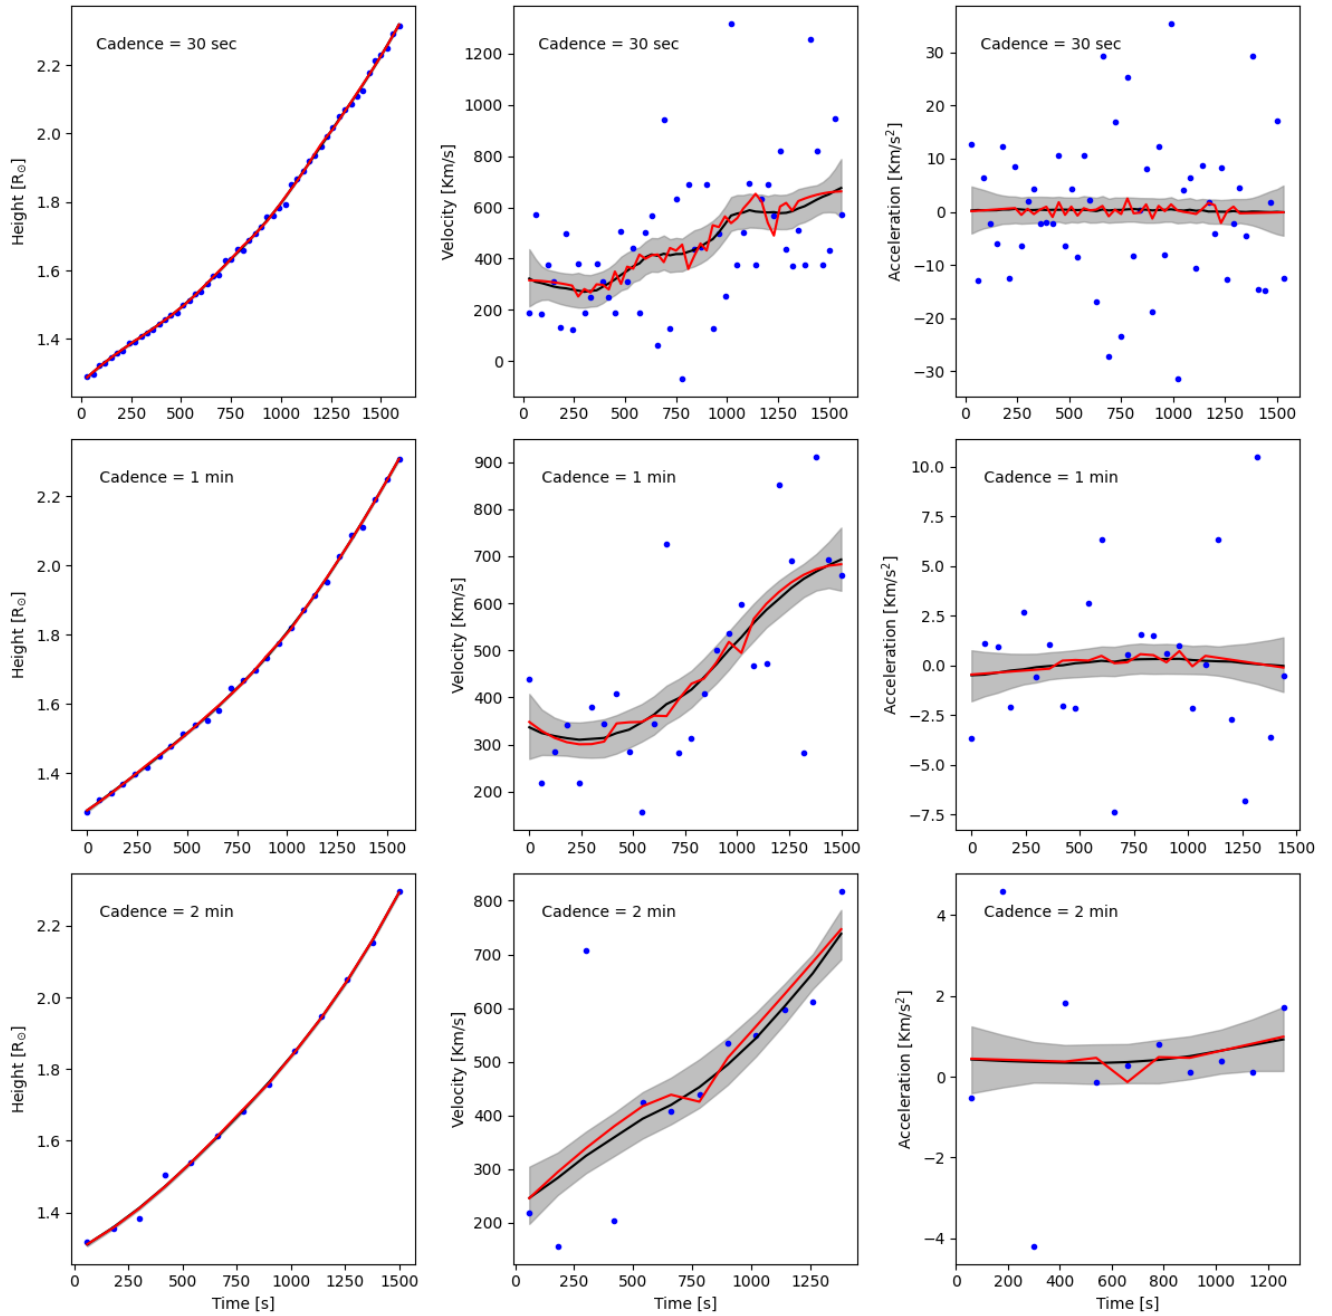

**Figure S14.** A complete kinematic profile of the CME observed on January 10, 2022. (a) represents the bootstrapped Savitzky-Golay filter applied height-time plot for each cadence (from top to bottom). (b) and (c) represents the corresponding velocity and acceleration plot, respectively. The blue dot represents (a) the height measurement taken using K-Cor coronagraph and (b) and (c) corresponding numerically derivative velocity and acceleration. The red line represents the fitted curve. The black line represents the median value, and the grey-shaded region depicts the interquartile range.

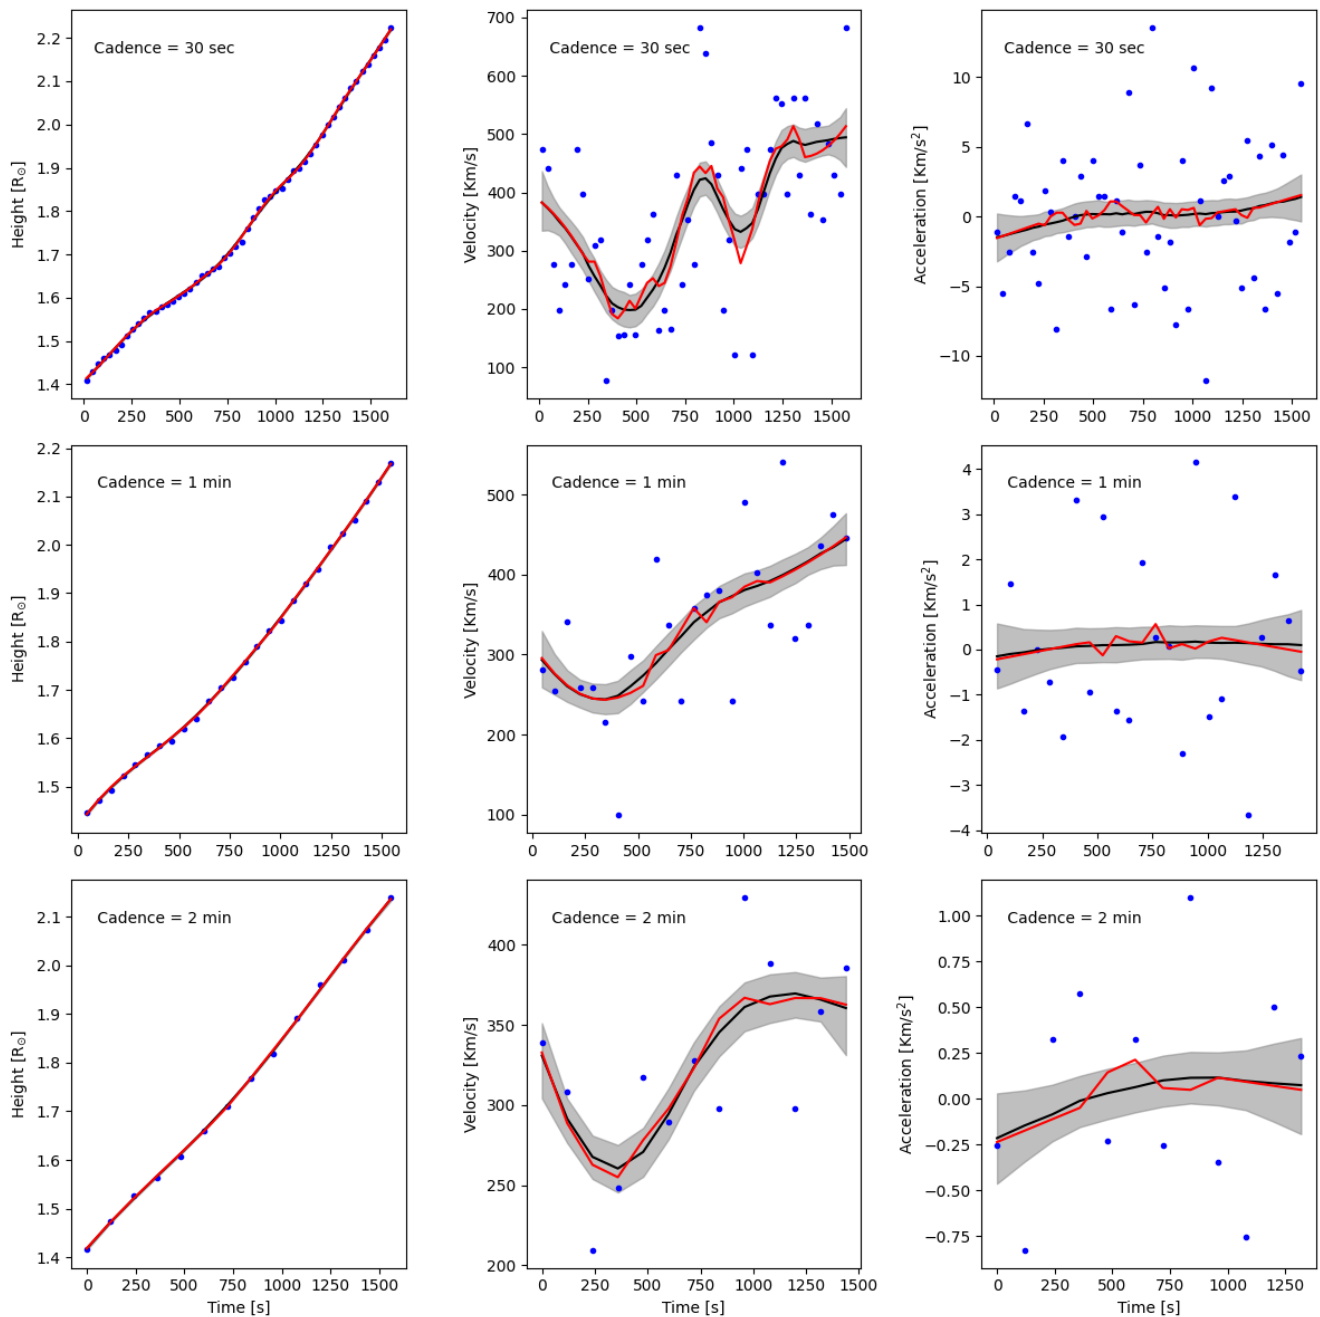

**Figure S15.** A complete kinematic profile of the CME observed on October 10, 2021. (a) represents the bootstrapped Savitzky-Golay filter applied height-time plot for each cadence (from top to bottom). (b) and (c) represents the corresponding velocity and acceleration plot, respectively. The blue dot represents (a) the height measurement taken using K-Cor coronagraph and (b) and (c) corresponding numerically derivative velocity and acceleration. The red line represents the fitted curve. The black line represents the median value, and the grey-shaded region depicts the interquartile range.

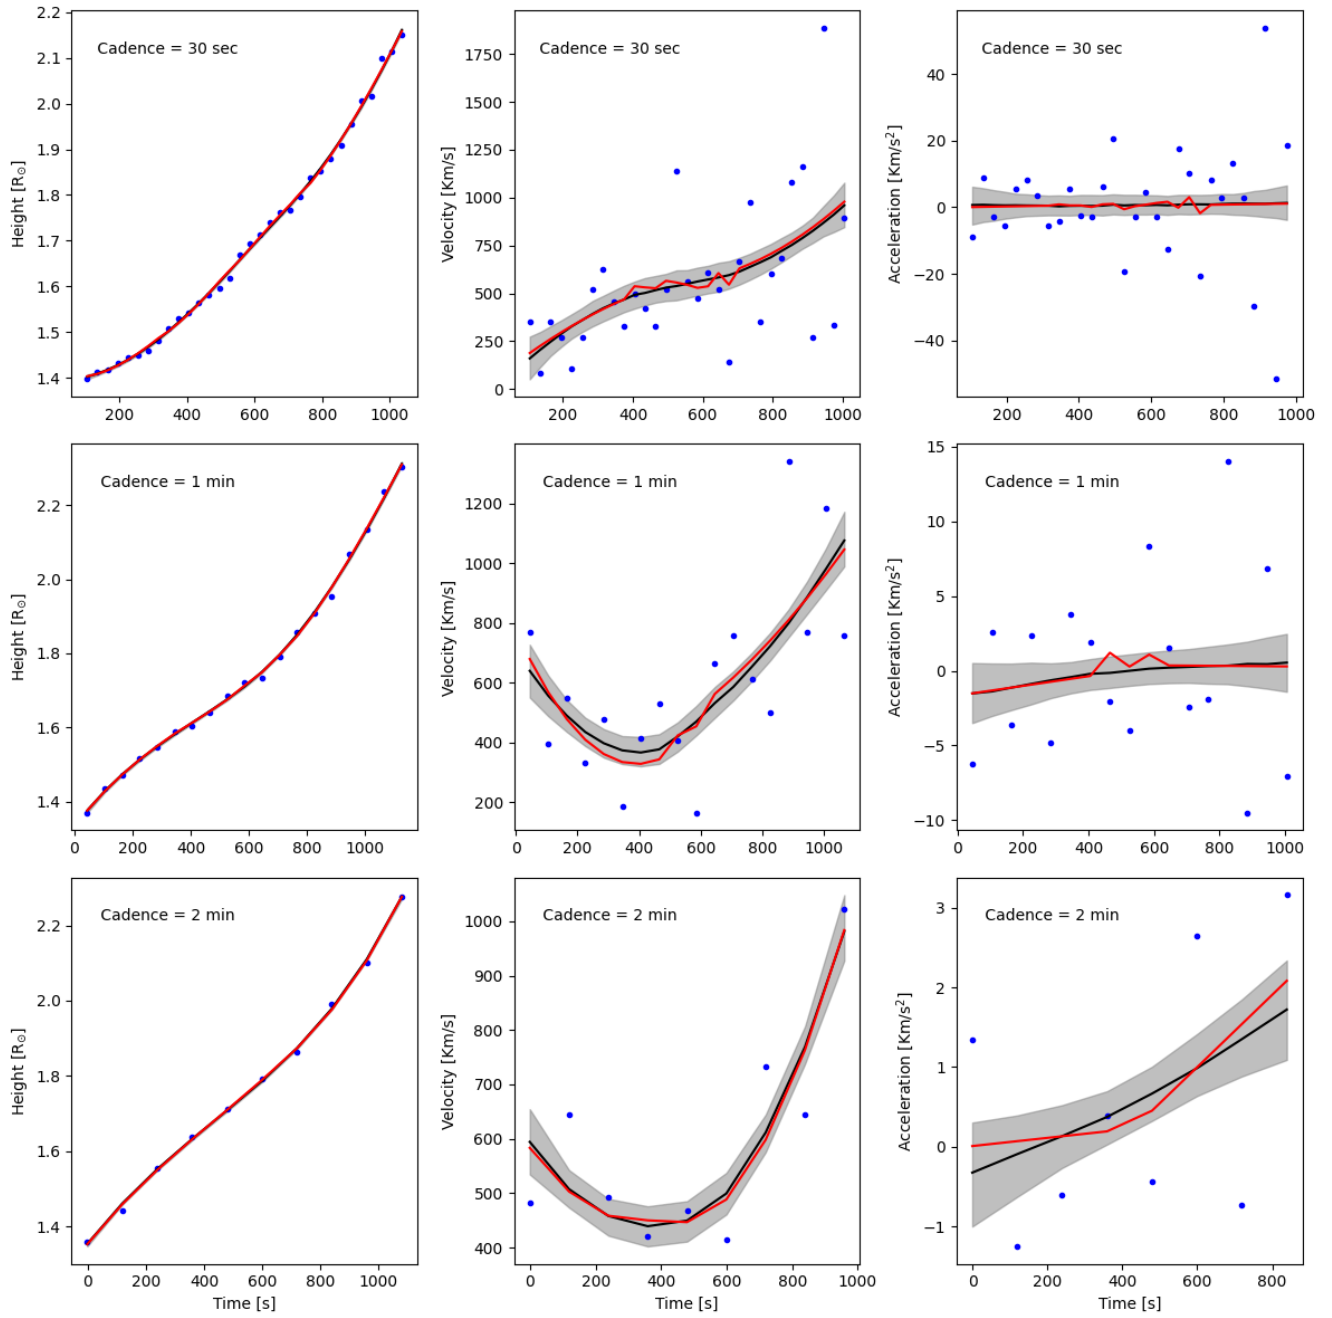

**Figure S16.** A complete kinematic profile of the CME observed on July 31, 2022. (a) represents the bootstrapped Savitzky-Golay filter applied height-time plot for each cadence (from top to bottom). (b) and (c) represents the corresponding velocity and acceleration plot, respectively. The blue dot represents (a) the height measurement taken using K-Cor coronagraph and (b) and (c) corresponding numerically derivative velocity and acceleration. The red line represents the fitted curve. The black line represents the median value, and the grey-shaded region depicts the interquartile range.



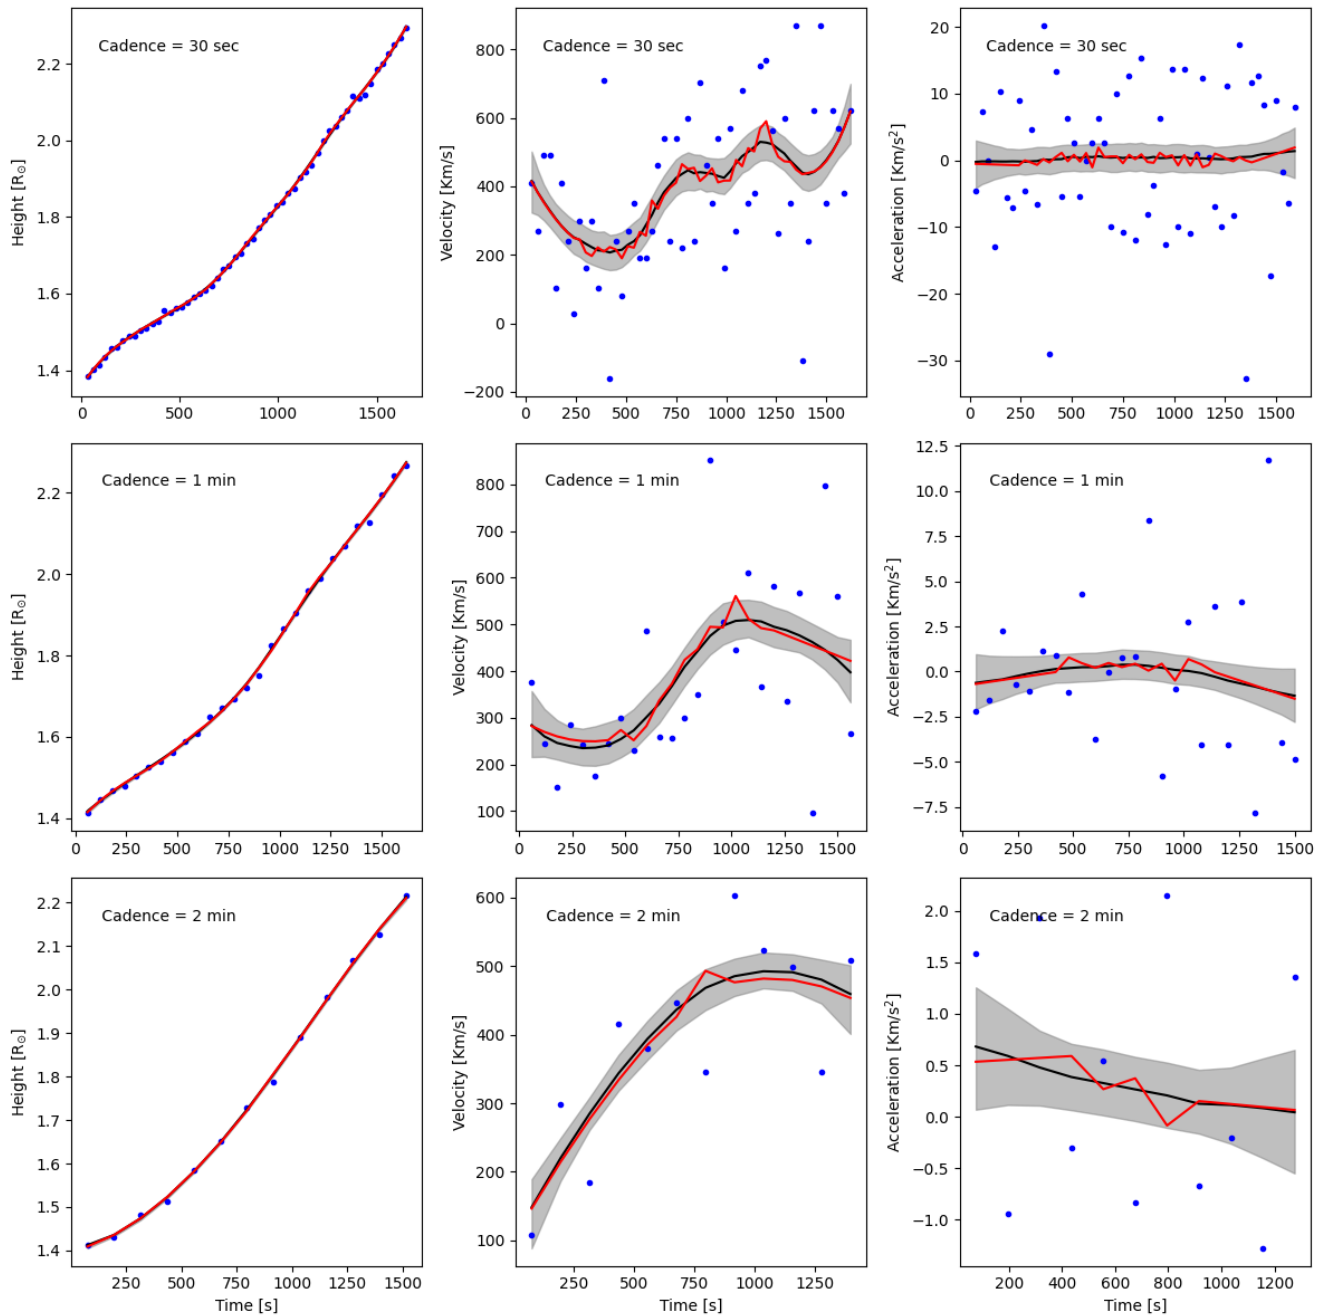

**Figure S17.** A complete kinematic profile of the CME observed on November 05, 2014. (a) represents the bootstrapped Savitzky-Golay filter applied height-time plot for each cadence (from top to bottom). (b) and (c) represents the corresponding velocity and acceleration plot, respectively. The blue dot represents (a) the height measurement taken using K-Cor coronagraph and (b) and (c) corresponding numerically derivative velocity and acceleration. The red line represents the fitted curve. The black line represents the median value, and the grey-shaded region depicts the interquartile range.

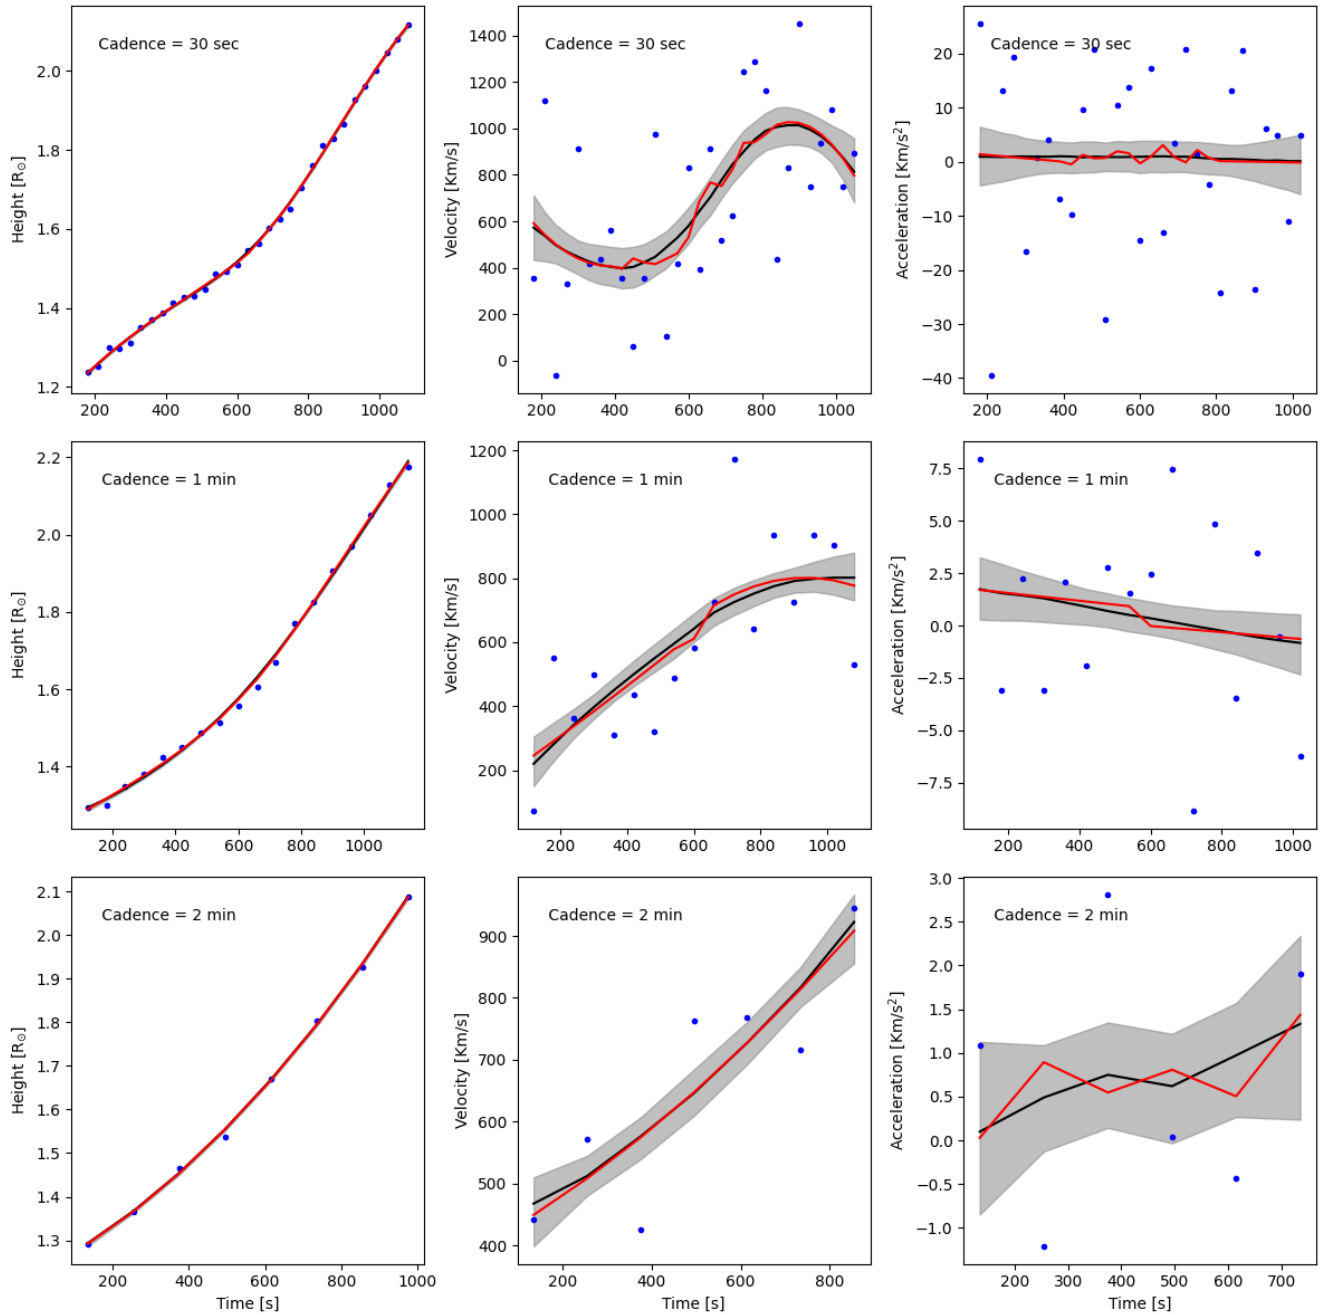

**Figure S18.** A complete kinematic profile of the CME observed on May 07, 2021. (a) represents the bootstrapped Savitzky-Golay filter applied height-time plot for each cadence (from top to bottom). (b) and (c) represents the corresponding velocity and acceleration plot, respectively. The blue dot represents (a) the height measurement taken using K-Cor coronagraph and (b) and (c) corresponding numerically derivative velocity and acceleration. The red line represents the fitted curve. The black line represents the median value, and the grey-shaded region depicts the interquartile range.
